# Supplementary material for: A Model of the Fed's View on Inflation
Source: arXiv:2006.14110 ancillary file (2020-06-25)
Supplement: Supplementary file 1 [file OnlineAppendix.pdf]

# ONLINE APPENDIX FOR A Model of the Fed's View on Inflation

Thomas Hasenzagl<sup>1</sup>, Filippo Pellegrino<sup>2</sup>, Lucrezia Reichlin<sup>3</sup>, and Giovanni Ricco<sup>4</sup>

<sup>1</sup>*University of Minnesota*

<sup>2</sup>*London School of Economics and Political Science*

<sup>3</sup>*London Business School, Now-Casting Economics, and CEPR*

<sup>4</sup>*University of Warwick, OFCE-SciencesPo, and CEPR*

First draft: December 2017

## Contents

|          |                                                                                          |           |
|----------|------------------------------------------------------------------------------------------|-----------|
| <b>A</b> | <b>Metropolis-Within-Gibbs</b>                                                           | <b>2</b>  |
| A.1      | Algorithm . . . . .                                                                      | 2         |
| <b>B</b> | <b>Posteriors of all parameters</b>                                                      | <b>6</b>  |
| <b>C</b> | <b>Robustness to Priors</b>                                                              | <b>10</b> |
| <b>D</b> | <b>Building up the Model</b>                                                             | <b>12</b> |
| D.1      | Model A: small-scale model with AR(1) cycles and without dynamic heterogeneity . . . . . | 12        |
| D.2      | Model B: Model A with ARMA(2,1) cycles . . . . .                                         | 17        |
| D.3      | Model C: Model B with EP cycle . . . . .                                                 | 21        |
| D.4      | Model D: Model C with employment and core inflation . . . . .                            | 25        |
| D.5      | Model E: Model D with University of Michigan inflation expectations . . . . .            | 29        |
| <b>E</b> | <b>Employment-to-Population Ratio</b>                                                    | <b>33</b> |
| <b>F</b> | <b>Global Activity</b>                                                                   | <b>37</b> |
| F.1      | Correlation of Cycles with Global Activity Indicators . . . . .                          | 37        |
| F.2      | A Model with Global Indicators . . . . .                                                 | 38        |
| <b>G</b> | <b>Priors for the Long-Run</b>                                                           | <b>42</b> |

## Appendix A Metropolis-Within-Gibbs

Starting with the work of [Beveridge and Nelson \(1981\)](#), [Harvey \(1985\)](#), and [Clark \(1987\)](#) several methodologies have been suggested in the literature to estimate trend-cycle models with unobserved components. As discussed in [Harvey et al. \(2007\)](#), frequentist techniques tend to deliver inaccurate estimates and – as a result – implausible cycles and trends, due to large estimation uncertainty. Conversely, Bayesian methods, which allow for the incorporation of a-priori knowledge into the model estimation, make it possible to consistently estimate both univariate and multivariate trend-cycle decompositions via efficient numerical methods.

In estimating our model we adopt a Metropolis-Within-Gibbs algorithm. However, since this approach tends to have slow performances in large dimensions, we run a simulation smoother only after the burn-in period to gain computational speed. In fact, during the burn-in period, we only employ a Kalman filter with exact diffuse initial conditions to estimate the likelihood function, as described in [Koopman and Durbin \(2000\)](#) and [Durbin and Koopman \(2012\)](#). This significantly increases the speed of the estimation which, given the large state-space of our model, is useful.

### A.1 Algorithm

The algorithm is structured in two blocks: (1) a Partially Adaptive Metropolis (e.g., [Herbst and Schorfheide, 2015](#)) step for the estimation of the state-space parameters, (2) a Gibbs sampler to draw the unobserved states conditional on the model parameters. In a Partially Adaptive Metropolis the variance covariance matrix,  $\Sigma$ , of the candidate distribution is generated in an initialisation step.

#### Algorithm: Metropolis-Within-Gibbs

##### Initialisation

For  $s = 1, \dots, n_s$  ( $n_s = 40000$ )

1. *Metropolis Algorithm*

- i. Draw a candidate vector for the unbounded parameters  $(\theta_*)$ , from a multivariate normal distribution with mean  $\theta_{s-1}$  and variance  $\omega\mathbb{I}$ , where  $\omega$  is a scaling constant used to get an acceptance rate between 25% and 35%
- ii. Set

$$\theta_s = \begin{cases} \theta_* & \text{with probability } \eta \\ \theta_{s-1} & \text{with probability } 1 - \eta \end{cases} \quad (1)$$

for

$$\eta = \min \left( 1, \frac{p(y | f(\theta_*)^{-1}) p(f(\theta_*)^{-1}) J(\theta_*)}{p(y | f(\theta_{s-1})^{-1}) p(f(\theta_{s-1})^{-1}) J(\theta_{s-1})} \right) \quad (2)$$

2. Discard the first  $s = 1, \dots, n_0$  ( $n_0 = 20000$ ) draws of  $\theta_s$ .

## Recursion

1. *Metropolis Algorithm*

Set  $\Sigma$  to the sample covariance of the chain of  $\theta_s$ , ( $s = \{n_0, \dots, n_s\}$ ), from the Initialisation step.

For  $q = 1, \dots, n_q$  ( $n_q = 20000$ )

- i. Draw a candidate vector for the parameters  $(\theta_*)$ , from a multivariate normal distribution with mean  $\theta_{q-1}$  and variance  $\omega\Sigma$ , where  $\omega$  is set to have an acceptance rate between 25% and 35%
- ii. Set

$$\theta_q = \begin{cases} \theta_* & \text{with probability } \eta \\ \theta_{q-1} & \text{with probability } 1 - \eta \end{cases} \quad (3)$$

where  $\eta$  is defined as in the Initialisation step.

2. *Gibbs sampling*

For  $n_q > n_\emptyset$  for  $n_\emptyset = 10000$  (burn-in period), apply the univariate approach for multivariate time series of [Koopman and Durbin \(2000\)](#) to the simulation smoother proposed in [Durbin and Koopman \(2002\)](#) to sample the

unobserved states, conditional on the parameters. In doing so, we follow the refinement proposed in [Jarociński \(2015\)](#).

3. Discard the first  $q = 1, \dots, n_\emptyset$  draws of  $\theta_q$ .

**Jacobian** Most of these parameters are constrained (or bounded) in their support (e.g. the variances of the shocks are greater than zero). The standard approach used to tackle this problem is to transform the bounded parameters ( $\Theta$ ) so that the support of the transformed parameters ( $\theta$ ) is unbounded. Our Metropolis algorithm draws the model parameters in the unbounded space in order to avoid a-priori rejections and to obtain a more efficient estimation routine.<sup>1</sup> The following transformations have been applied to parameters with Normal, Inverse-Gamma and Uniform priors, respectively:

$$\begin{aligned}\theta_j^N &= \Theta_j^N \\ \theta_j^{IG} &= \ln(\Theta_j^{IG} - a_j) \\ \theta_j^U &= \ln\left(\frac{\Theta_j^U - a_j}{b_j - \Theta_j^U}\right)\end{aligned}$$

Where  $a_j$  and  $b_j$  are the lower and the upper bounds for the  $j$ -th parameter. These transformations are functions  $f(\Theta) = \theta$ , with inverses  $f(\theta)^{-1} = \Theta$  given by:

$$\begin{aligned}\Theta_j^N &= \theta_j^N \\ \Theta_j^{IG} &= \exp(\theta_j^{IG}) + a_j \\ \Theta_j^U &= \frac{a_j + b_j \exp(\theta_j^U)}{1 + \exp(\theta_j^U)}\end{aligned}$$

---

<sup>1</sup>This description uses the same notation and a similar approach to the one described in [Warne \(2008\)](#)

These transformations must be taken into account when evaluating the natural logarithm of the prior densities in (2), by adding the Jacobians of the transformations of the variables:

$$\begin{aligned}\ln \left( \frac{d\Theta_j^N}{d\theta_j^N} \right) &= 0 \\ \ln \left( \frac{d\Theta_j^{IG}}{d\theta_j^{IG}} \right) &= \theta_j^{IG} \\ \ln \left( \frac{d\Theta_j^U}{d\theta_j^U} \right) &= \ln(b_j - a_j) + \theta_j^U - 2 \ln(1 + \exp(\theta_j^U))\end{aligned}$$

**Code** The code is written in Julia (<http://julialang.org>) and it has been parallelised since it is computationally expensive.

## Appendix B Posteriors of all parameters

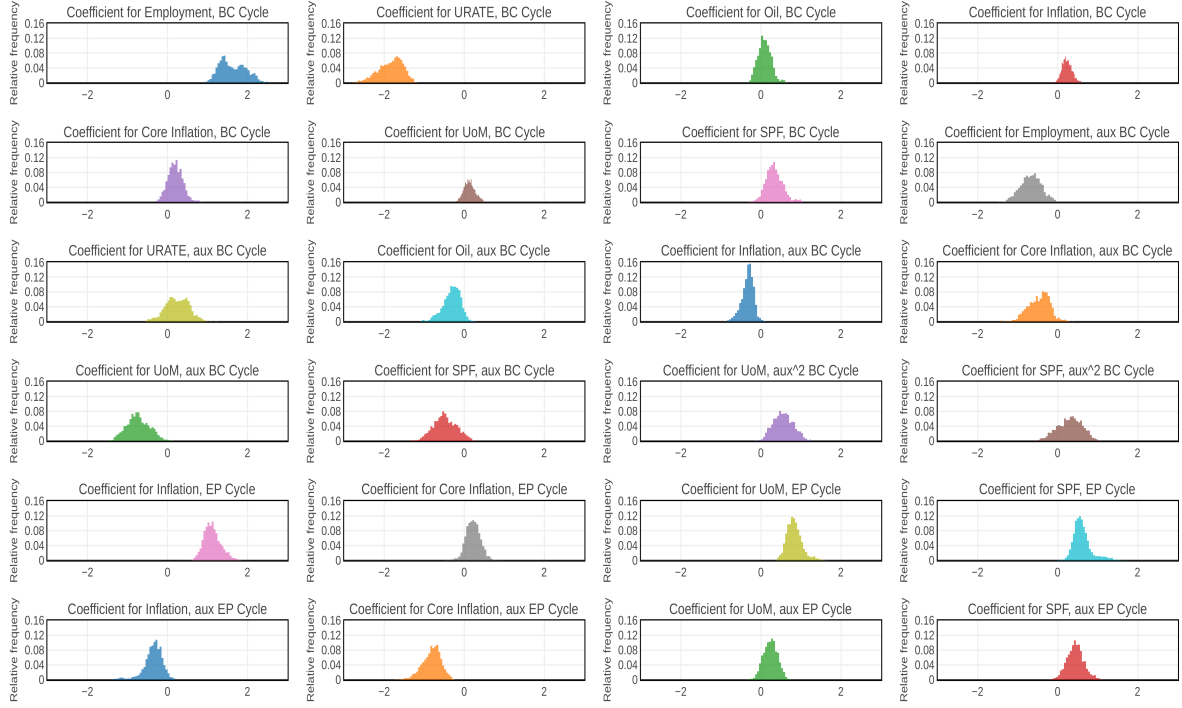

Figure 1: Coefficients

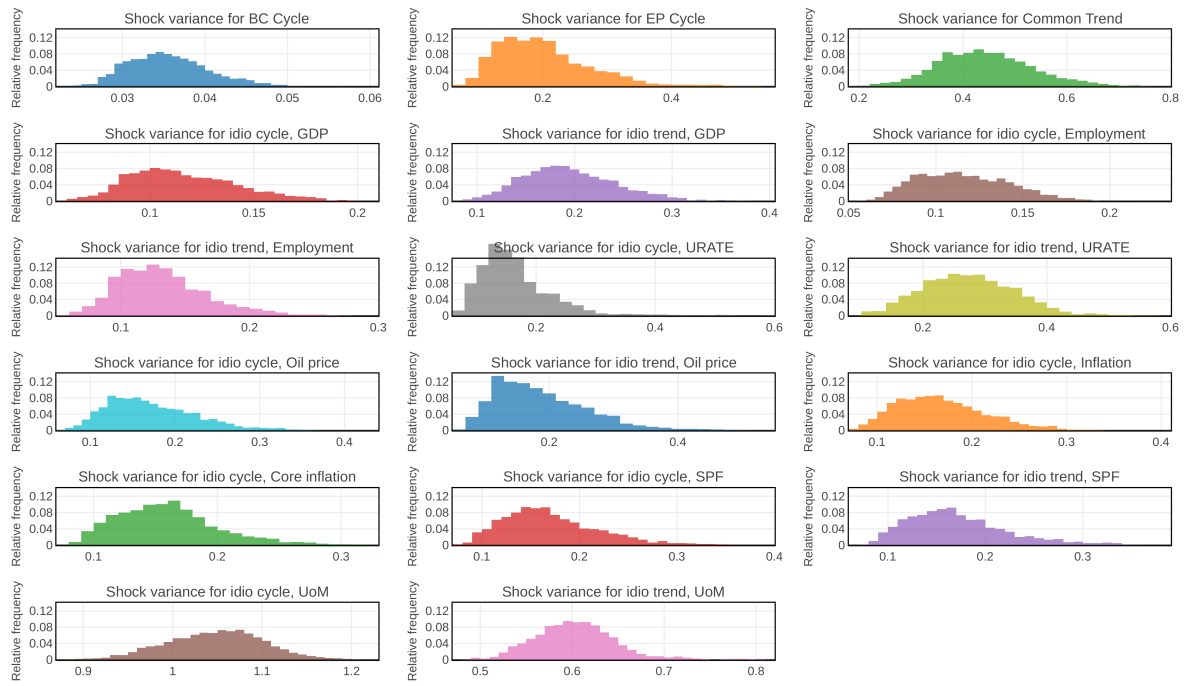

**Figure 2: Variance of shocks**

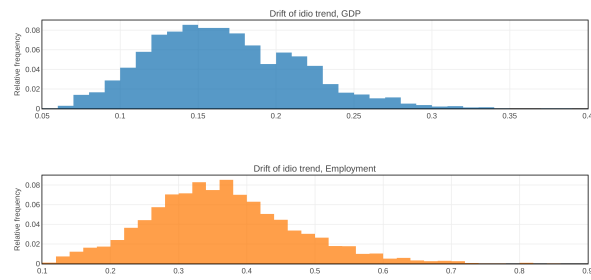

**Figure 3: Drifts**

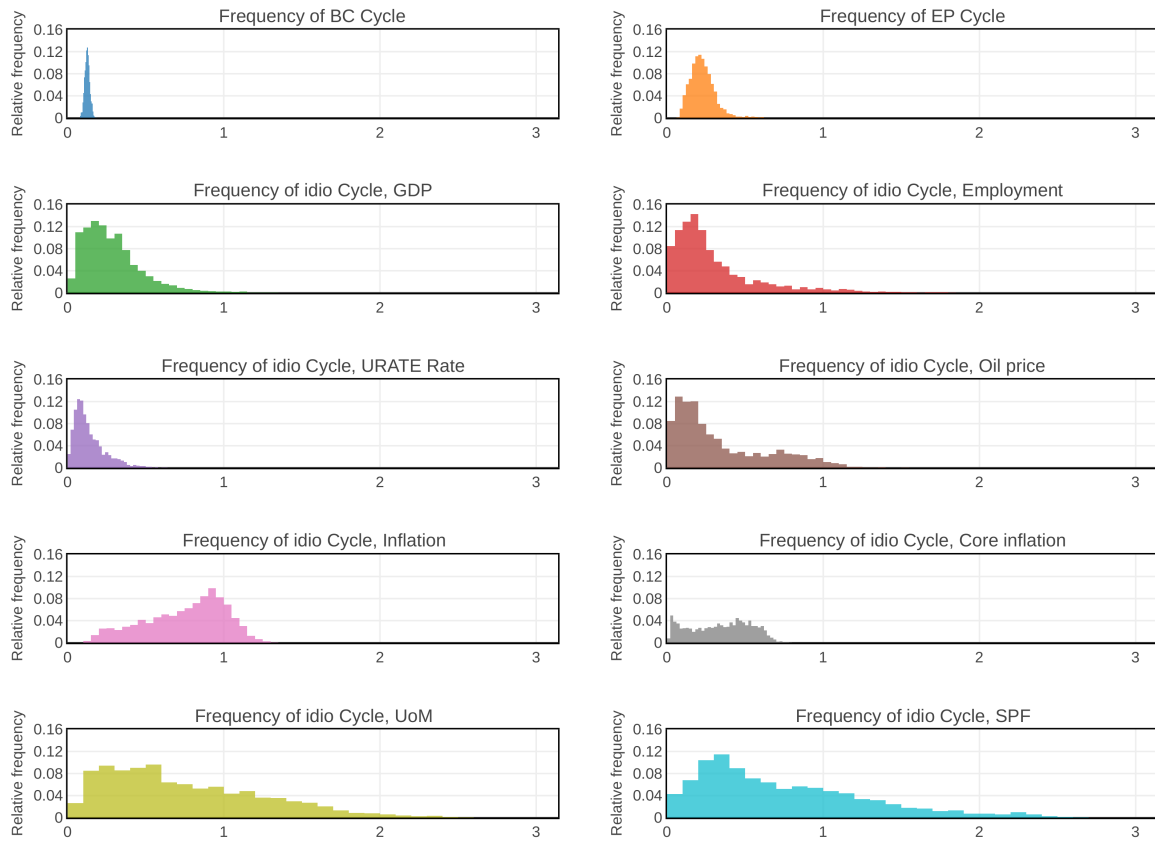

**Figure 4:** Frequency of cycles



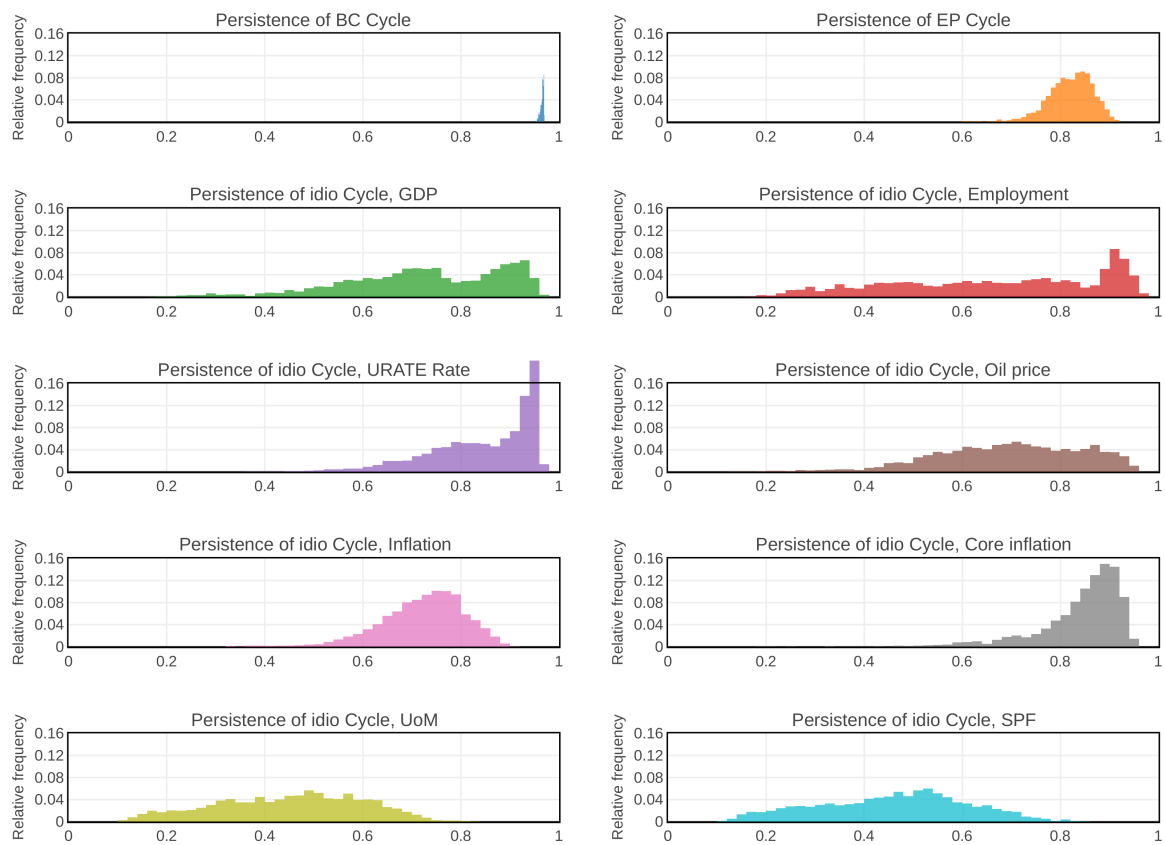

**Figure 5:** Persistence of cycles

## Appendix C Robustness to Priors

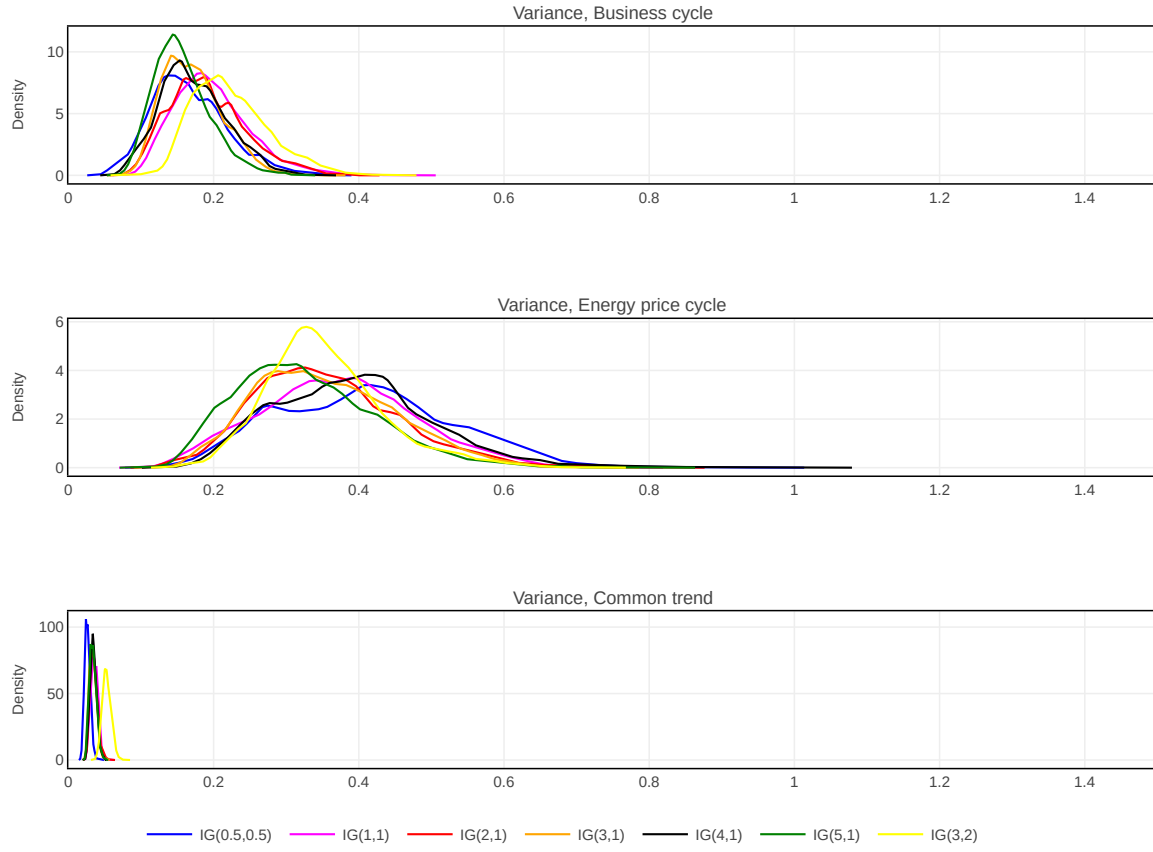

**Figure 6:** The chart reports the posterior distributions of the variance of the shocks to the business cycle (top), energy price cycle (middle), and common trend (bottom) when the inverse gamma priors of those variances have different shape and scale parameters.

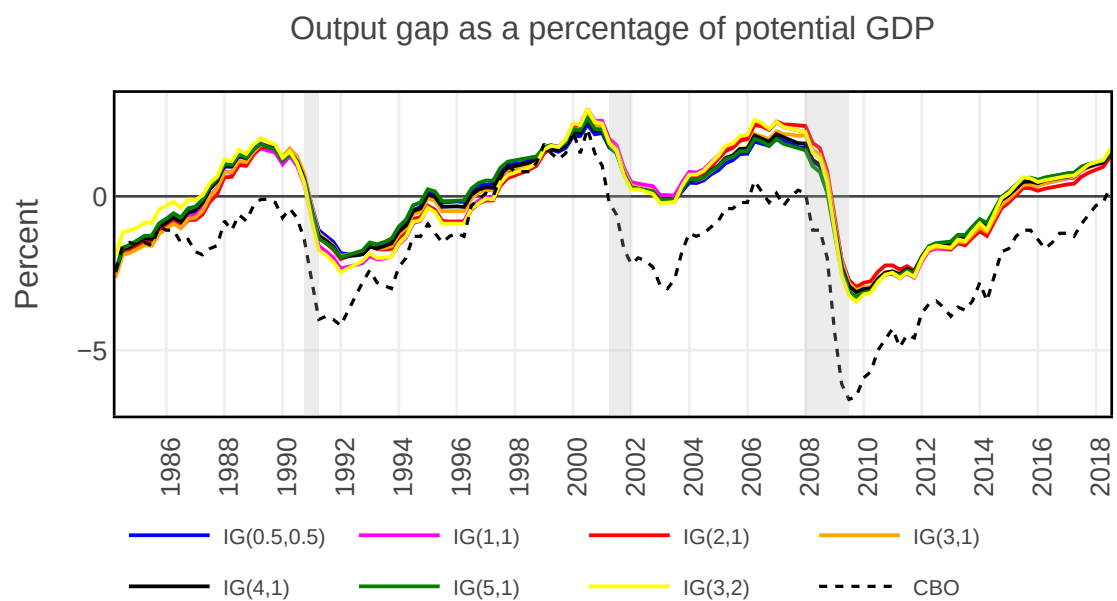

**Figure 7:** The chart reports the median of the output gap when the priors for the variance of the shocks to the common components are inverse gamma priors with different shape and scale parameters. The chart also reports the output gap from the CBO.

## Appendix D Building up the Model

### D.1 Model A: small-scale model with AR(1) cycles and without dynamic heterogeneity

For this model we used the data reported in the table below.

**Table 1:** Data and transformations

| Variable          | Symbol                | Mnemonic | Transformation |
|-------------------|-----------------------|----------|----------------|
| Real GDP          | $y_t$                 | $y$      | Levels         |
| Unemployment rate | $u_t$                 | $u$      | Levels         |
| Oil price         | $oil_t$               | $oil$    | Levels         |
| CPI inflation     | $\pi_t$               | $\pi$    | YoY            |
| SPF: Expected CPI | $F_t^{spf} \pi_{t+4}$ | $spf$    | Levels         |

**Note:** The table lists the macroeconomic variables used in the empirical model. ‘SPF: Expected CPI’ is the Survey of Professional Forecasters, 4-quarters ahead expected CPI inflation rate. The oil price is the West Texas Intermediate Spot oil price.

The observation equation for this model is:

$$\begin{pmatrix} y_t \\ u_t \\ oil_t \\ \pi_t \\ F_t^{spf} \pi_{t+4} \end{pmatrix} = \begin{pmatrix} 1 & 0 \\ \delta_{u,1} & 0 \\ \delta_{oil,1} & 0 \\ \delta_{\pi,1} & \phi_\pi \\ \delta_{spf,1} + \delta_{spf,2}L & \phi_{spf} \end{pmatrix} \begin{pmatrix} \hat{\psi}_t \\ \mu_t^\pi \end{pmatrix} + \begin{pmatrix} \psi_t^y \\ \psi_t^u \\ \psi_t^{oil} \\ \psi_t^\pi \\ \psi_t^{spf} \end{pmatrix} + \begin{pmatrix} \mu_t^y \\ \mu_t^u \\ \mu_t^{oil} \\ 0 \\ \mu_t^{spf} \end{pmatrix} \quad (4)$$

where  $\phi_\pi$  and  $\phi_{spf}$  are normalised to have unitary loading of inflation and inflation expectations on trend inflation.<sup>2</sup> The cycles are modelled as stationary AR(1) with a U(-0.97,

<sup>2</sup>In the empirical model, the series are standardised so that the standard deviations of their first differences are equal to one. For this reason, we normalise  $\phi_\pi$  and  $\phi_{spf}$  to the reciprocal of the standard deviation of the first difference of the respective variable.

0.97) prior on the autoregressive coefficients.

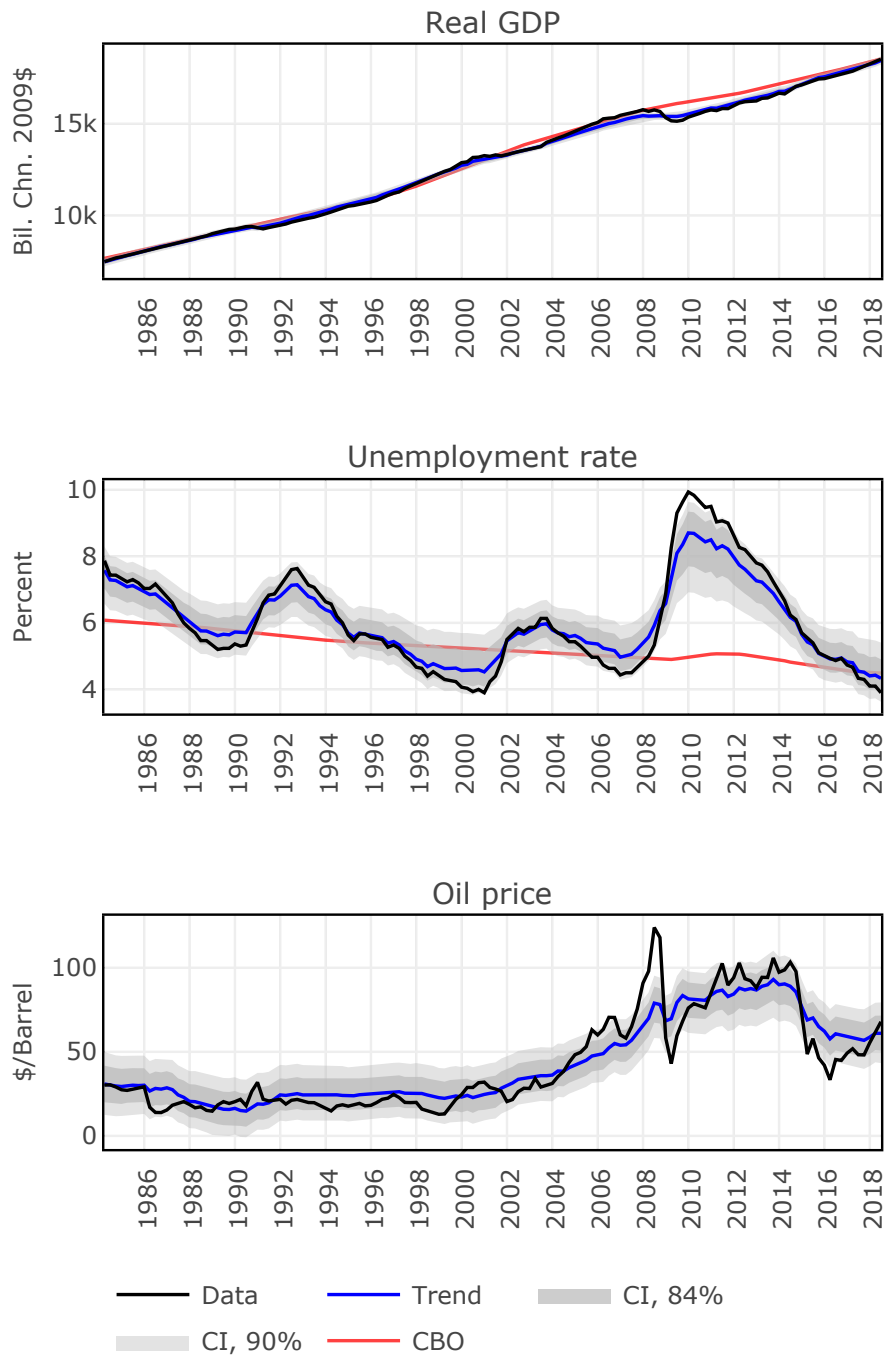

**Figure 8:** Independent trends of output, unemployment, and oil prices (in blue), with coverage intervals at 68% coverage (dark shade) and 90% coverage (light shade), as estimated by the model. The chart also reports the measures of potential outputs and NAIRU estimated by the CBO (in red).

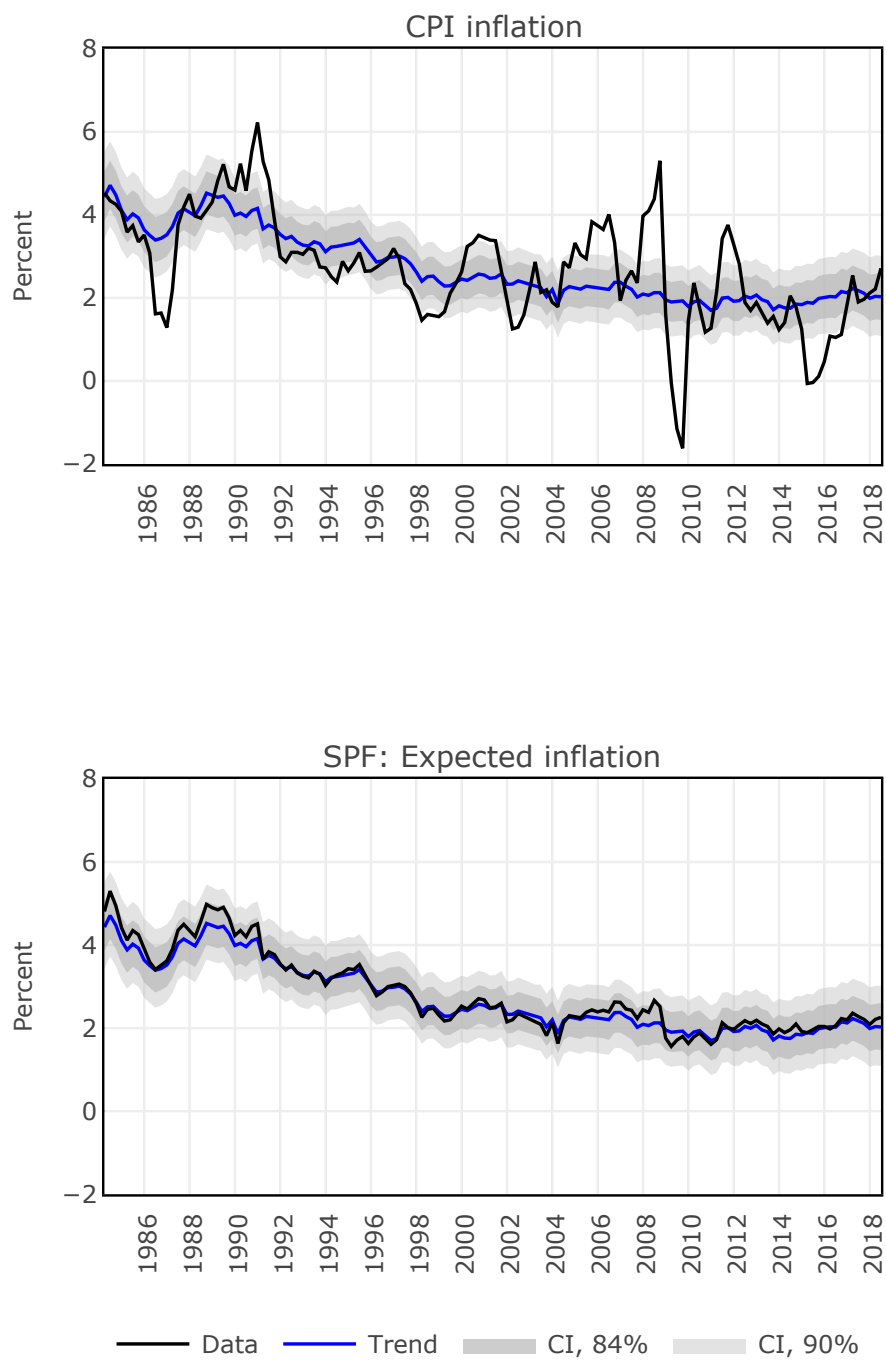

**Figure 9:** Trend common to CPI inflation and SPF inflation expectations (in blue), with coverage intervals at 68% coverage (dark shade) and 90% coverage (light shade), as estimated by the model.

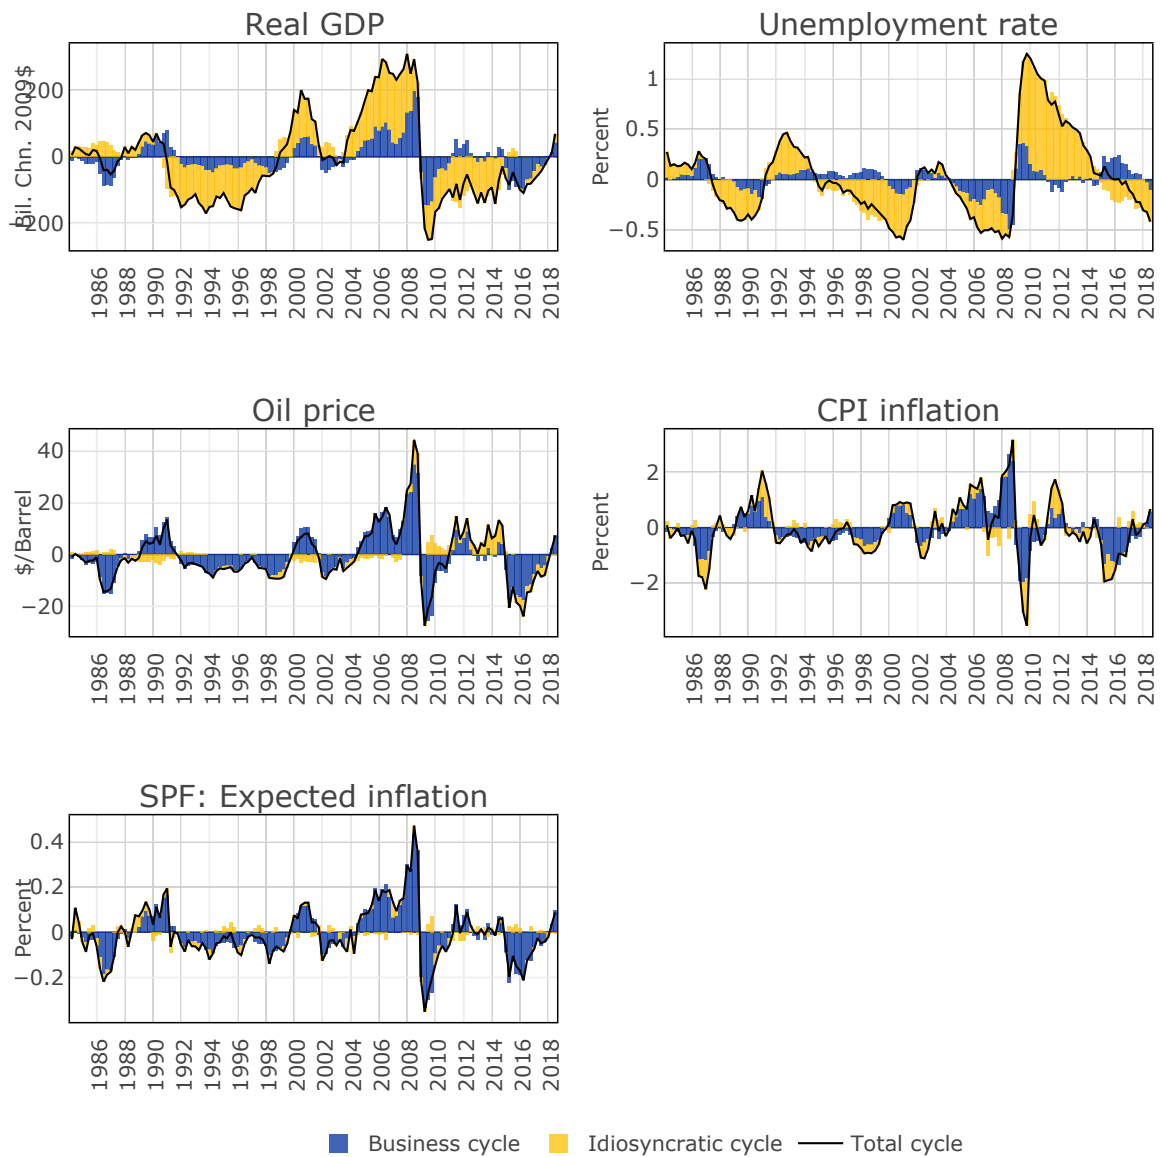

**Figure 10:** Historical decomposition of the cycles, as estimated by the model. The chart reports the Business cycle (in blue), and idiosyncratic cycle (in yellow).



## **D.2 Model B: Model A with ARMA(2,1) cycles**

Same data and observation equation used for the model A. Cycles are modelled as in the baseline trend-cycle model in the main text - i.e. as ARMA(2,1).

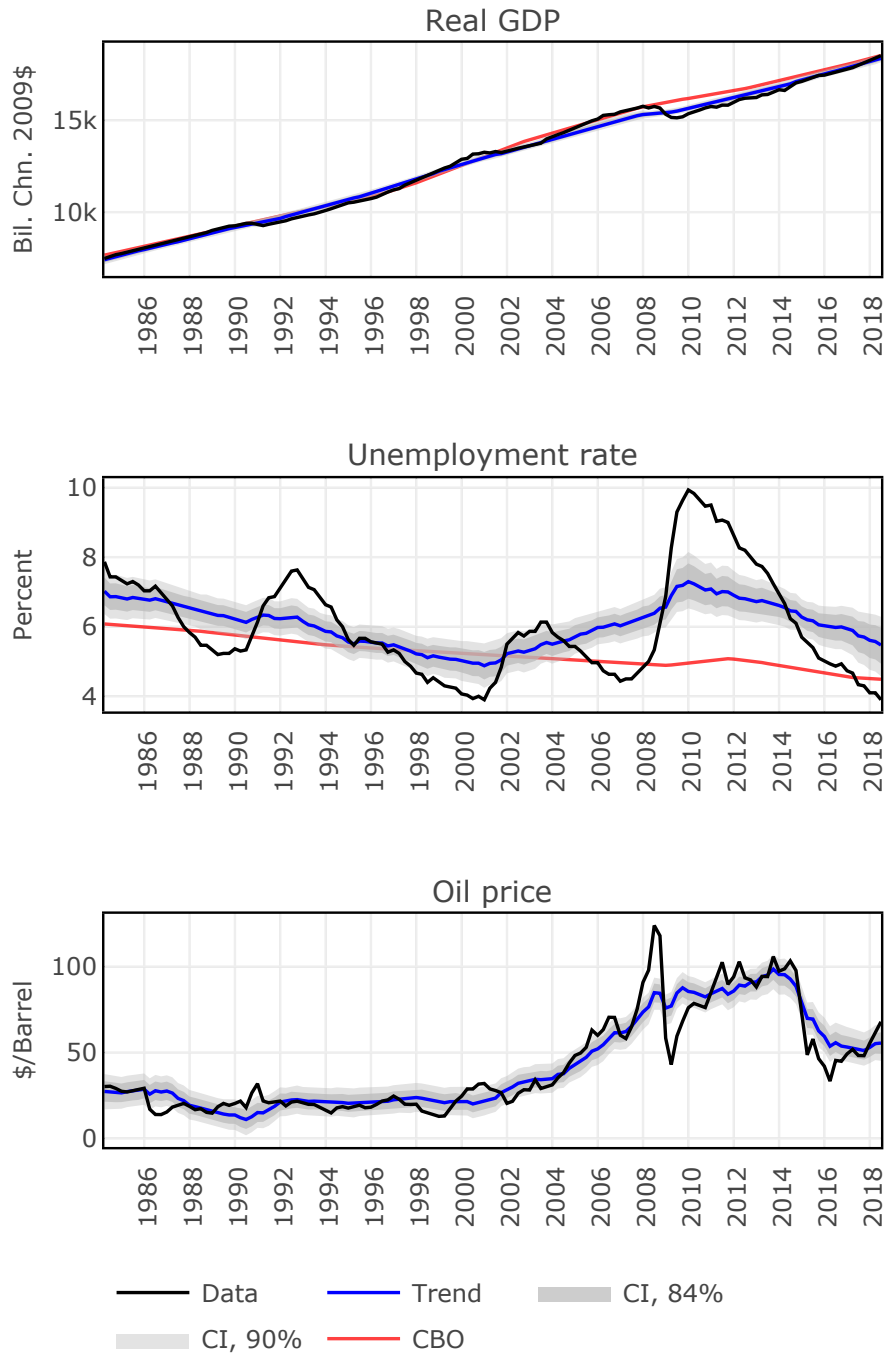

**Figure 11:** Independent trends of output, unemployment, and oil prices (in blue), with coverage intervals at 68% coverage (dark shade) and 90% coverage (light shade), as estimated by the model. The chart also reports the measures of potential outputs and NAIRU estimated by the CBO (in red).

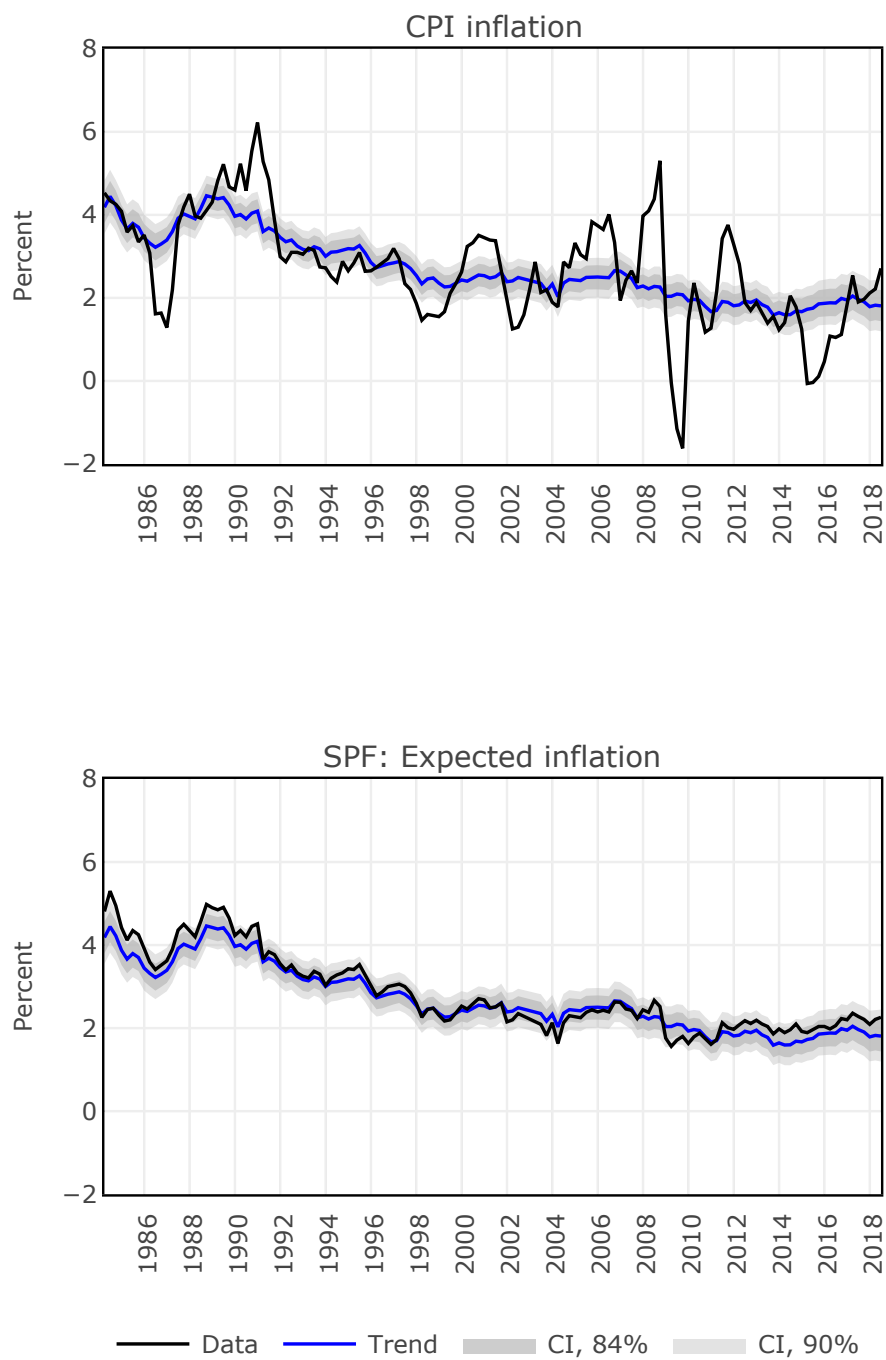

**Figure 12:** Trend common to CPI inflation and SPF inflation expectations (in blue), with coverage intervals at 68% coverage (dark shade) and 90% coverage (light shade), as estimated by the model.

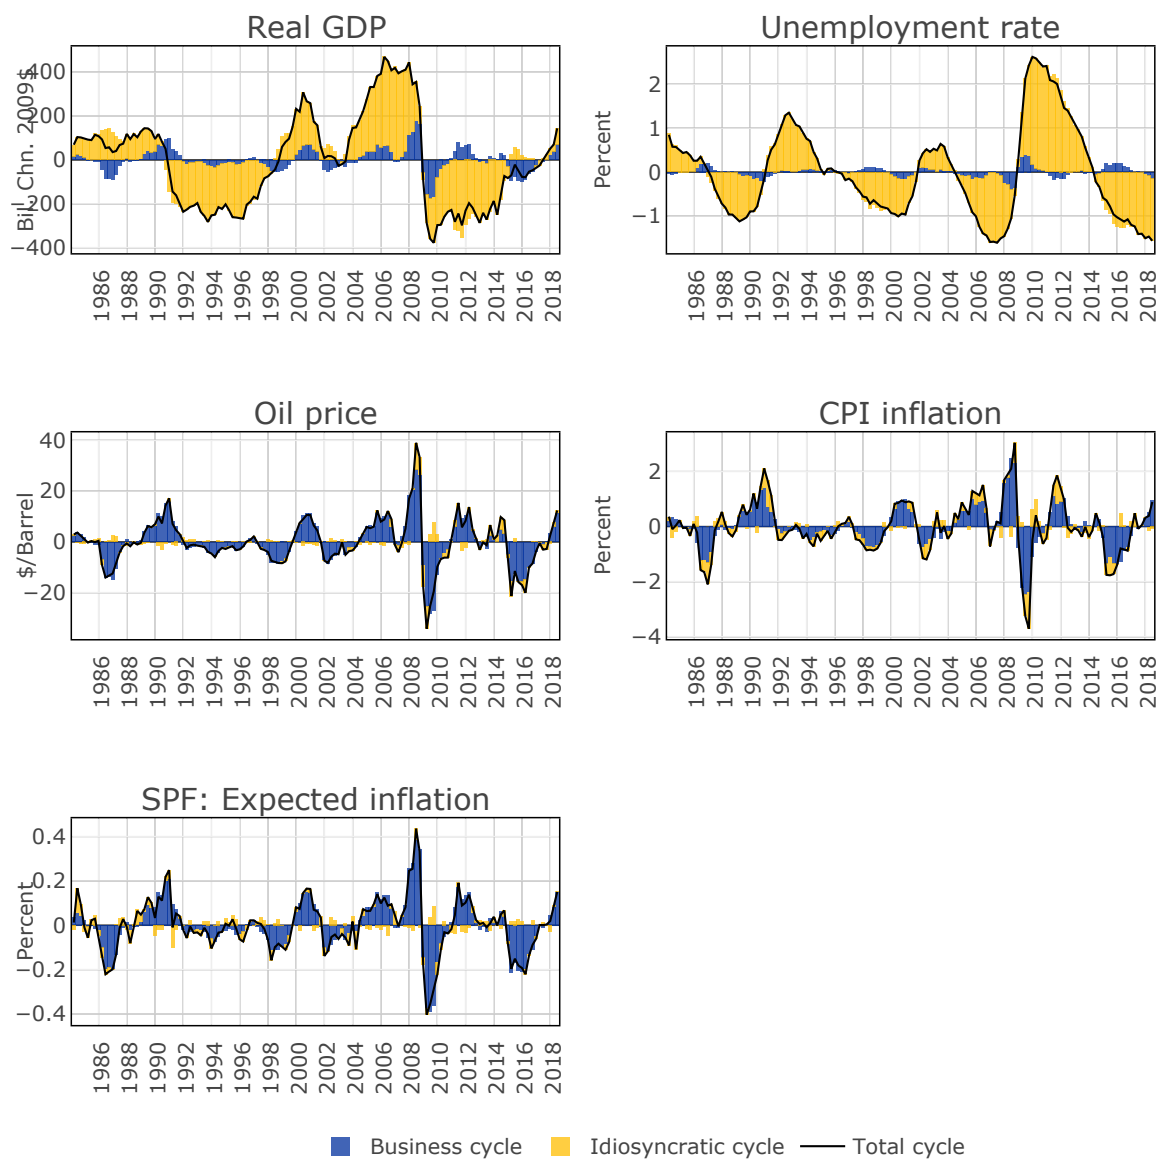

**Figure 13:** Historical decomposition of the cycles, as estimated by the model. The chart reports the Business cycle (in blue), and idiosyncratic cycle (in yellow).

### D.3 Model C: Model B with EP cycle

For this model we used the data reported in [Table 1](#). The observation equation for this model is:

$$\begin{pmatrix} y_t \\ u_t \\ oil_t \\ \pi_t \\ F_t^{spf} \pi_{t+4} \end{pmatrix} = \begin{pmatrix} 1 & 0 & 0 \\ \delta_{u,1} & 0 & 0 \\ \delta_{oil,1} & 1 & 0 \\ \delta_{\pi,1} & \gamma_{\pi,1} & \phi_{\pi} \\ \delta_{spf,1} + \delta_{spf,2}L & \gamma_{spf,1} & \phi_{spf} \end{pmatrix} \begin{pmatrix} \hat{\psi}_t \\ \psi_t^{EP} \\ \mu_t^{\pi} \end{pmatrix} + \begin{pmatrix} \psi_t^y \\ \psi_t^u \\ \psi_t^{oil} \\ \psi_t^{\pi} \\ \psi_t^{spf} \end{pmatrix} + \begin{pmatrix} \mu_t^y \\ \mu_t^u \\ \mu_t^{oil} \\ 0 \\ \mu_t^{spf} \end{pmatrix} \quad (5)$$

where  $\phi_{\pi}$  and  $\phi_{spf}$  are normalised to have unitary loading of inflation and inflation expectations on trend inflation.<sup>3</sup>

---

<sup>3</sup>In the empirical model, the series are standardised so that the standard deviations of their first differences are equal to one. For this reason, we normalise  $\phi_{\pi}$  and  $\phi_{spf}$  to the reciprocal of the standard deviation of the first difference of the respective variable.

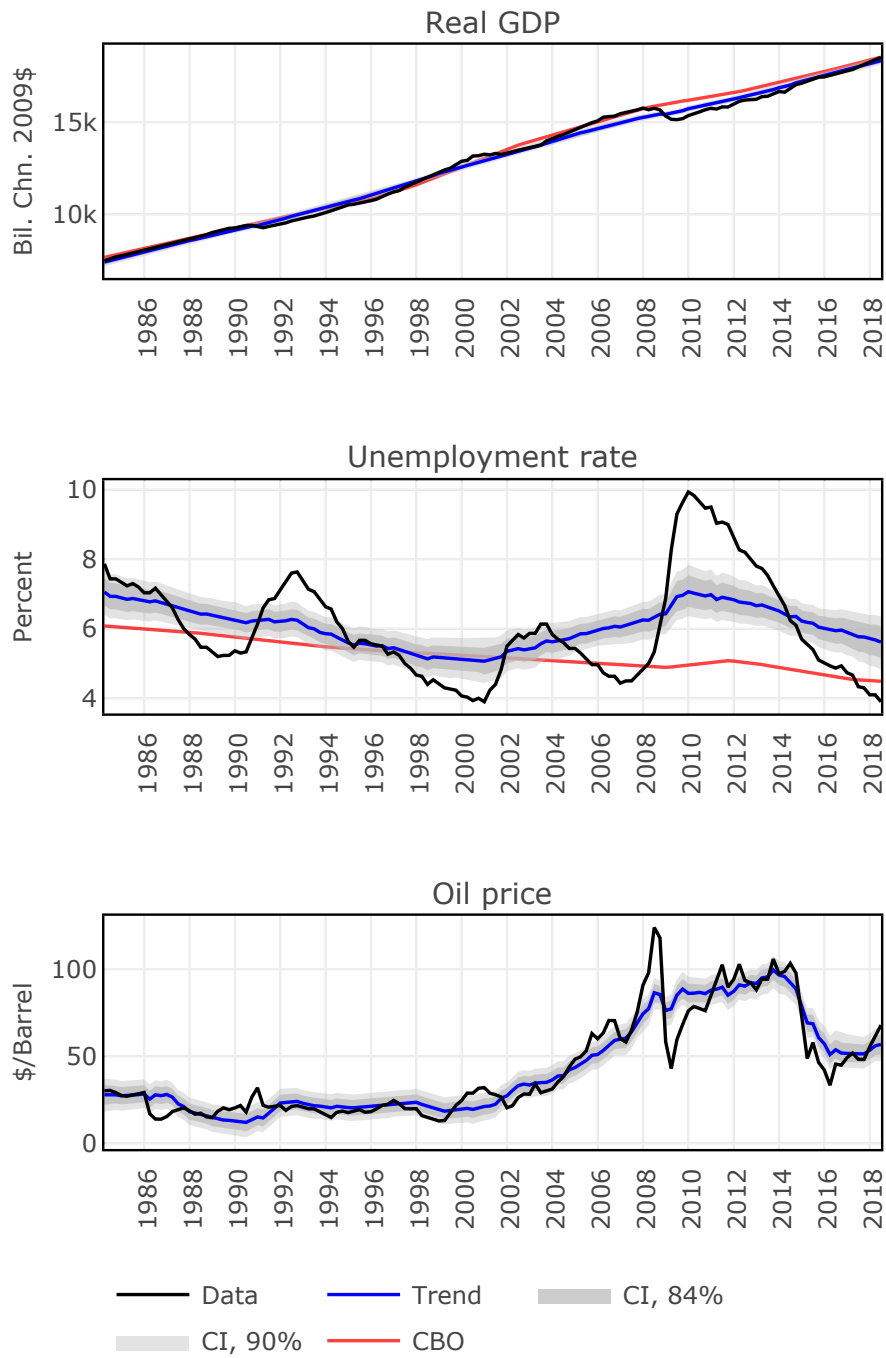

**Figure 14:** Independent trends of output, unemployment, and oil prices (in blue), with coverage intervals at 68% coverage (dark shade) and 90% coverage (light shade), as estimated by the model. The chart also reports the measures of potential outputs and NAIRU estimated by the CBO (in red).

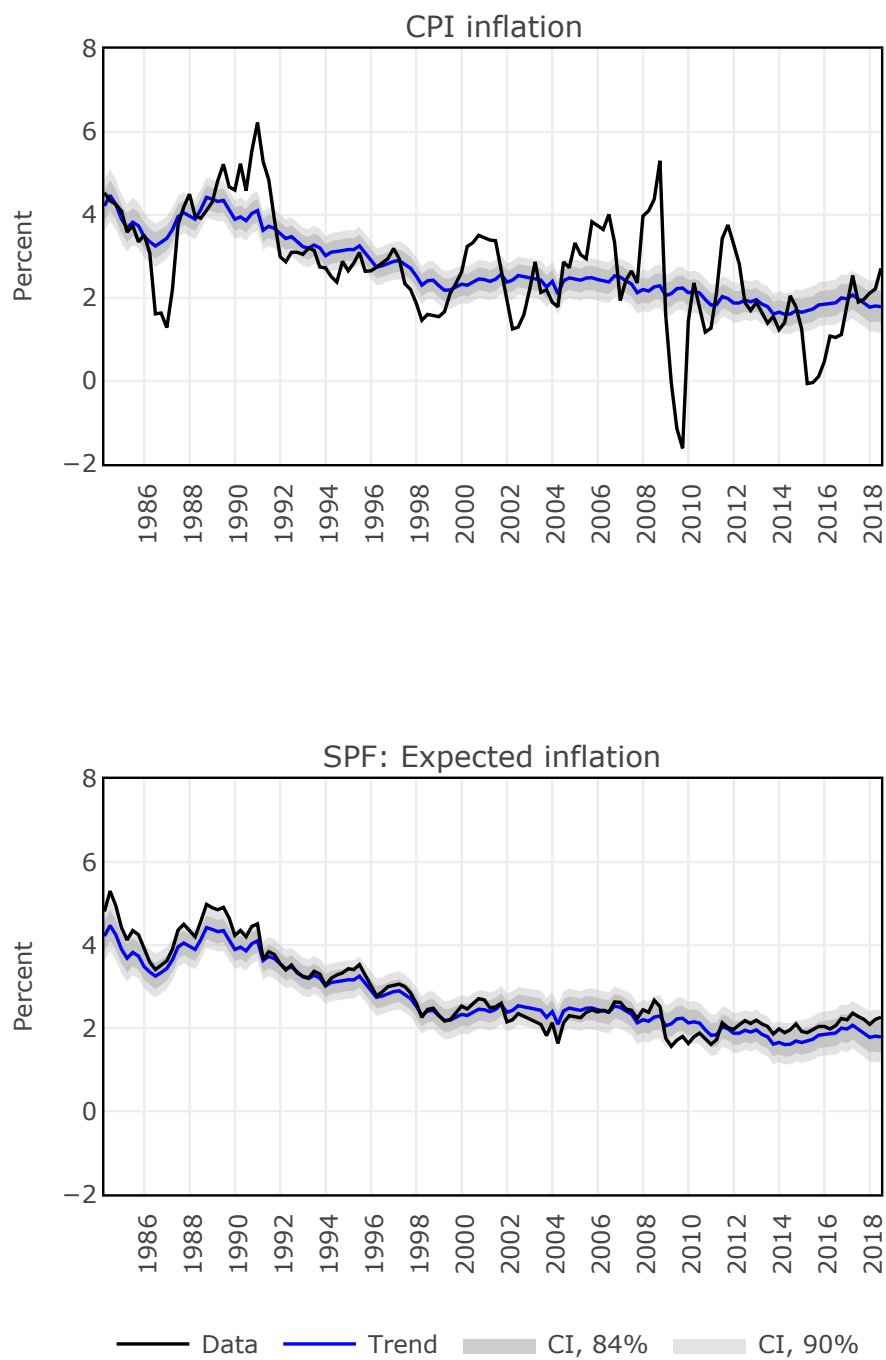

**Figure 15:** Trend common to CPI inflation and SPF inflation expectations (in blue), with coverage intervals at 68% coverage (dark shade) and 90% coverage (light shade), as estimated by the model.

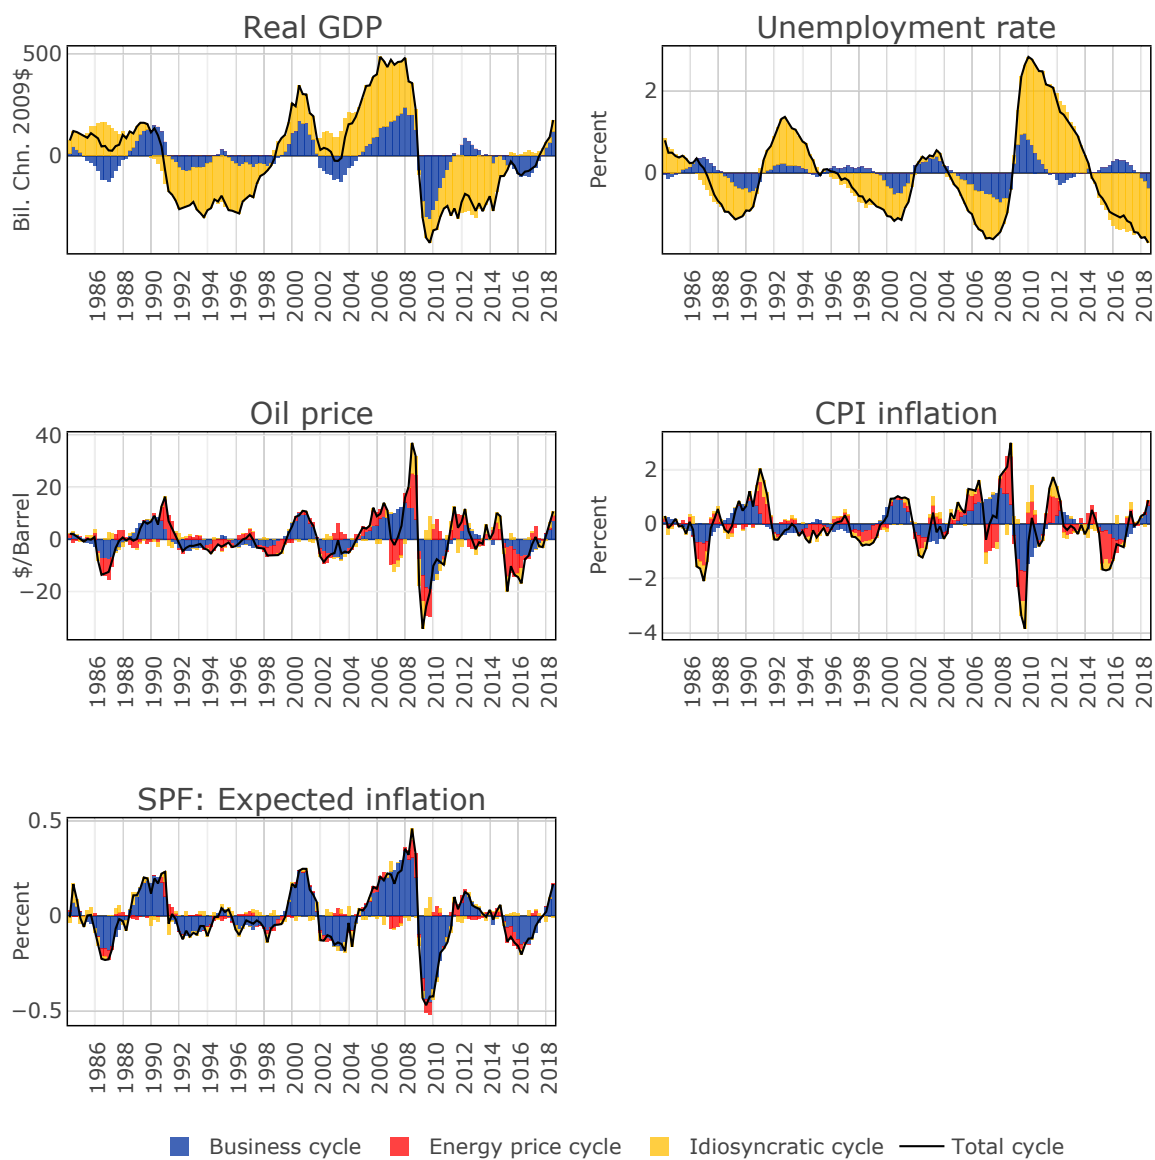

**Figure 16:** Historical decomposition of the cycles, as estimated by the model. The chart reports the Business cycle (in blue), Energy price cycle (in red), and idiosyncratic cycle (in yellow).



## D.4 Model D: Model C with employment and core inflation

For this model we used the data reported in the table below.

**Table 2:** Data and transformations

| Variable           | Symbol                | Mnemonic | Transformation |
|--------------------|-----------------------|----------|----------------|
| Real GDP           | $y_t$                 | $y$      | Levels         |
| Employment         | $e_t$                 | $e$      | Levels         |
| Unemployment rate  | $u_t$                 | $u$      | Levels         |
| Oil price          | $oil_t$               | $oil$    | Levels         |
| CPI inflation      | $\pi_t$               | $\pi$    | YoY            |
| Core CPI inflation | $\pi_t^c$             | $\pi^c$  | YoY            |
| SPF: Expected CPI  | $F_t^{spf} \pi_{t+4}$ | $spf$    | Levels         |

**Note:** The table lists the macroeconomic variables used in the empirical model. ‘SPF: Expected CPI’ is the Survey of Professional Forecasters, 4-quarters ahead expected CPI inflation rate. The oil price is the West Texas Intermediate Spot oil price.

The observation equation for this model is:

$$\begin{pmatrix} y_t \\ e_t \\ u_t \\ oil_t \\ \pi_t \\ \pi_t^c \\ F_t^{spf} \pi_{t+4} \end{pmatrix} = \begin{pmatrix} 1 & 0 & 0 \\ \delta_{e,1} & 0 & 0 \\ \delta_{u,1} & 0 & 0 \\ \delta_{oil,1} & 1 & 0 \\ \delta_{\pi,1} & \gamma_{\pi,1} & \phi_{\pi} \\ \delta_{\pi^c,1} & \gamma_{\pi^c,1} & \phi_{\pi^c} \\ \delta_{spf,1} + \delta_{spf,2}L & \gamma_{spf,1} & \phi_{spf} \end{pmatrix} \begin{pmatrix} \hat{\psi}_t \\ \psi_t^{EP} \\ \mu_t^{\pi} \end{pmatrix} + \begin{pmatrix} \psi_t^y \\ \psi_t^e \\ \psi_t^u \\ \psi_t^{oil} \\ \psi_t^{\pi} \\ \psi_t^{\pi^c} \\ \psi_t^{spf} \end{pmatrix} + \begin{pmatrix} \mu_t^y \\ \mu_t^e \\ \mu_t^u \\ \mu_t^{oil} \\ 0 \\ 0 \\ \mu_t^{spf} \end{pmatrix} \quad (6)$$

where  $\phi_{\pi}$ ,  $\phi_{\pi^c}$  and  $\phi_{spf}$  are normalised to have unitary loading of inflation and inflation expectations on trend inflation.<sup>4</sup>

<sup>4</sup>In the empirical model, the series are standardised so that the standard deviations of their first differences are equal to one. For this reason, we normalise  $\phi_{\pi}$ ,  $\phi_{\pi^c}$  and  $\phi_{spf}$  to the reciprocal of the standard deviation of the first difference of the respective variable.

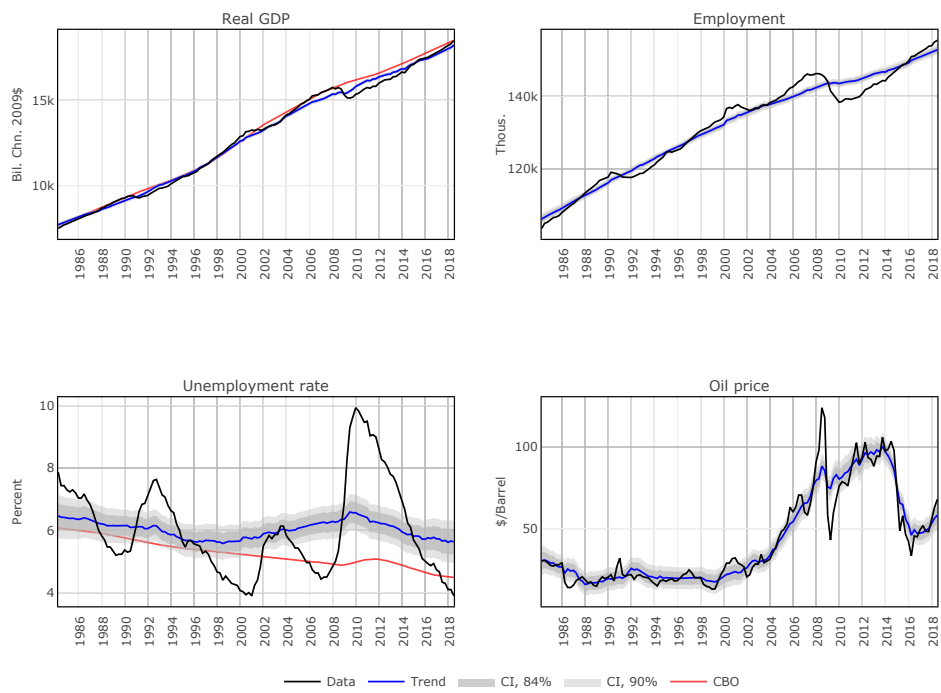

**Figure 17:** Independent trends of output, employment, unemployment, and oil prices (in blue), with coverage intervals at 68% coverage (dark shade) and 90% coverage (light shade), as estimated by the model. The chart also reports the measures of potential outputs and NAIRU estimated by the CBO (in red).

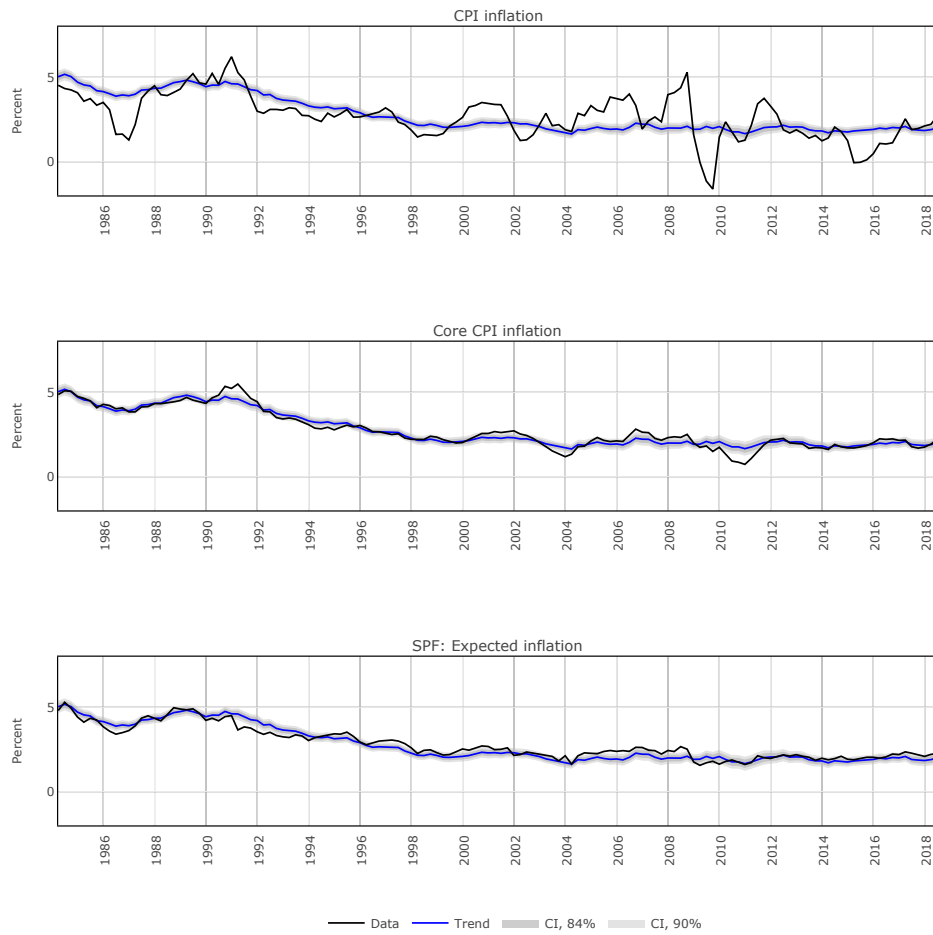

**Figure 18:** Trend common to CPI inflation, core CPI inflation, and inflation expectations (in blue), with coverage intervals at 68% coverage (dark shade) and 90% coverage (light shade), as estimated by the model.

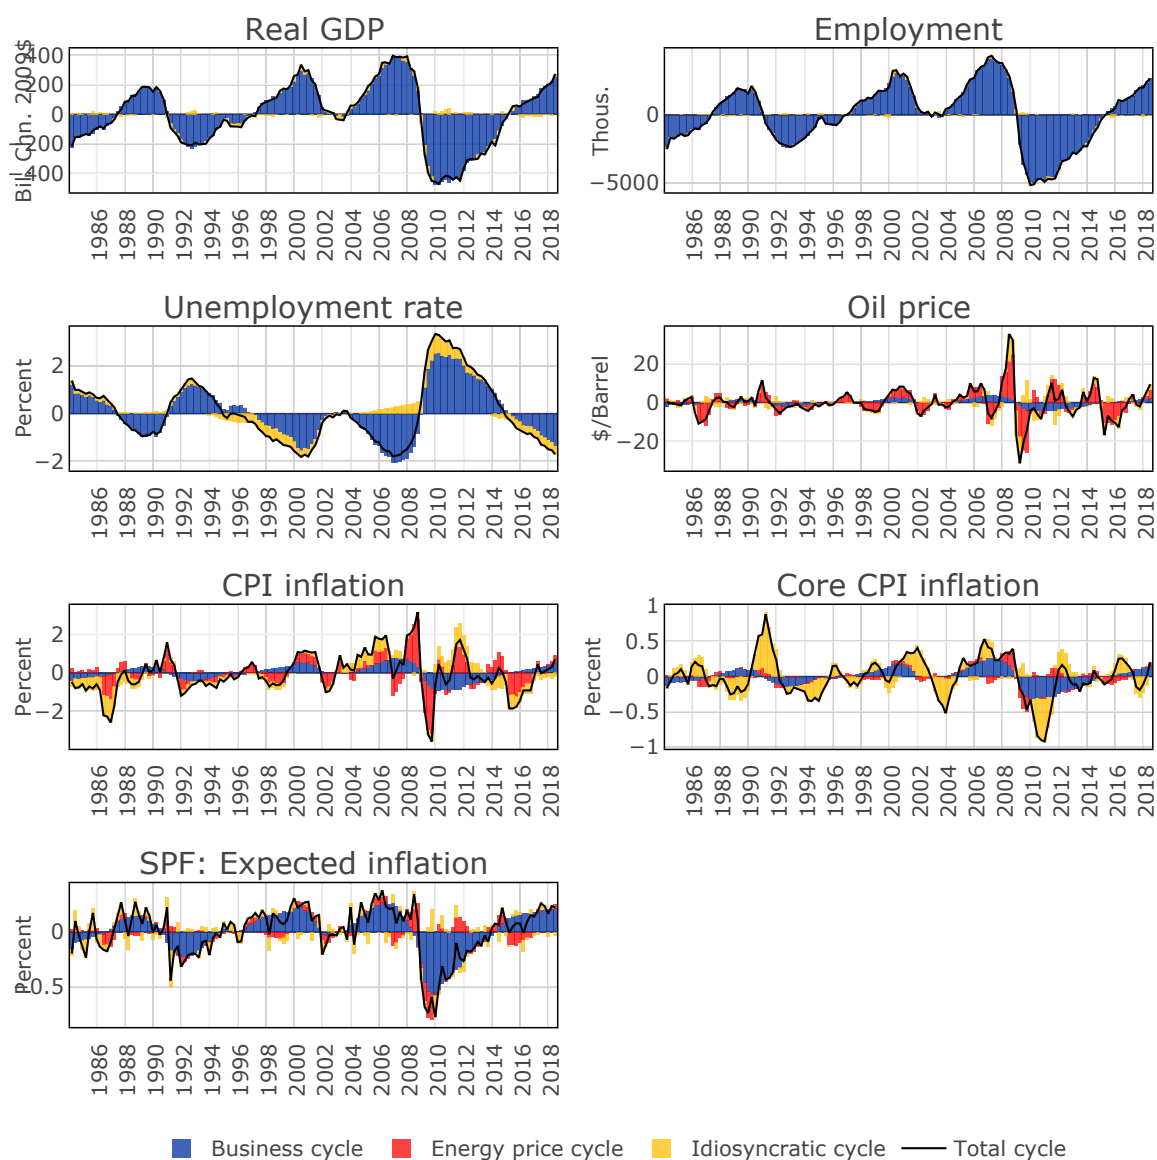

**Figure 19:** Historical decomposition of the cycles, as estimated by the model. The chart reports the Business cycle (in blue), Energy price cycle (in red), and idiosyncratic cycle (in yellow).

## D.5 Model E: Model D with University of Michigan inflation expectations

For this model we used the data reported in the table below.

**Table 3:** Data and transformations

| Variable                | Symbol                | Mnemonic | Transformation |
|-------------------------|-----------------------|----------|----------------|
| Real GDP                | $y_t$                 | $y$      | Levels         |
| Employment              | $e_t$                 | $e$      | Levels         |
| Unemployment rate       | $u_t$                 | $u$      | Levels         |
| Oil price               | $oil_t$               | $oil$    | Levels         |
| CPI inflation           | $\pi_t$               | $\pi$    | YoY            |
| Core CPI inflation      | $\pi_t^c$             | $\pi^c$  | YoY            |
| UoM: Expected inflation | $F_t^{uom} \pi_{t+4}$ | $uom$    | Levels         |
| SPF: Expected CPI       | $F_t^{spf} \pi_{t+4}$ | $spf$    | Levels         |

**Note:** The table lists the macroeconomic variables used in the empirical model. ‘UoM: Expected inflation’ is the University of Michigan, 12-months ahead expected inflation rate. ‘SPF: Expected CPI’ is the Survey of Professional Forecasters, 4-quarters ahead expected CPI inflation rate. The oil price is the West Texas Intermediate Spot oil price.

The observation equation for this model is:

$$\begin{pmatrix} y_t \\ e_t \\ u_t \\ oil_t \\ \pi_t \\ \pi_t^c \\ F_t^{uom} \pi_{t+4} \\ F_t^{spf} \pi_{t+4} \end{pmatrix} = \begin{pmatrix} 1 & 0 & 0 \\ \delta_{e,1} & 0 & 0 \\ \delta_{u,1} & 0 & 0 \\ \delta_{oil,1} & 1 & 0 \\ \delta_{\pi,1} & \gamma_{\pi,1} & \phi_{\pi} \\ \delta_{\pi^c,1} & \gamma_{\pi^c,1} & \phi_{\pi^c} \\ \delta_{uom,1} + \delta_{uom,2}L & \gamma_{uom,1} & \phi_{uom} \\ \delta_{spf,1} + \delta_{spf,2}L & \gamma_{spf,1} & \phi_{spf} \end{pmatrix} \begin{pmatrix} \hat{\psi}_t \\ \psi_t^{EP} \\ \mu_t^{\pi} \end{pmatrix} + \begin{pmatrix} \psi_t^y \\ \psi_t^e \\ \psi_t^u \\ \psi_t^{oil} \\ \psi_t^{\pi} \\ \psi_t^{\pi^c} \\ \psi_t^{uom} \\ \psi_t^{spf} \end{pmatrix} + \begin{pmatrix} \mu_t^y \\ \mu_t^e \\ \mu_t^u \\ \mu_t^{oil} \\ 0 \\ 0 \\ \mu_t^{uom} \\ \mu_t^{spf} \end{pmatrix} \quad (7)$$

where  $\phi_{\pi}$ ,  $\phi_{\pi^c}$ ,  $\phi_{uom}$  and  $\phi_{spf}$  are normalised to have unitary loading of inflation and inflation expectations on trend inflation.<sup>5</sup>

<sup>5</sup>In the empirical model, the series are standardised so that the standard deviations of their first

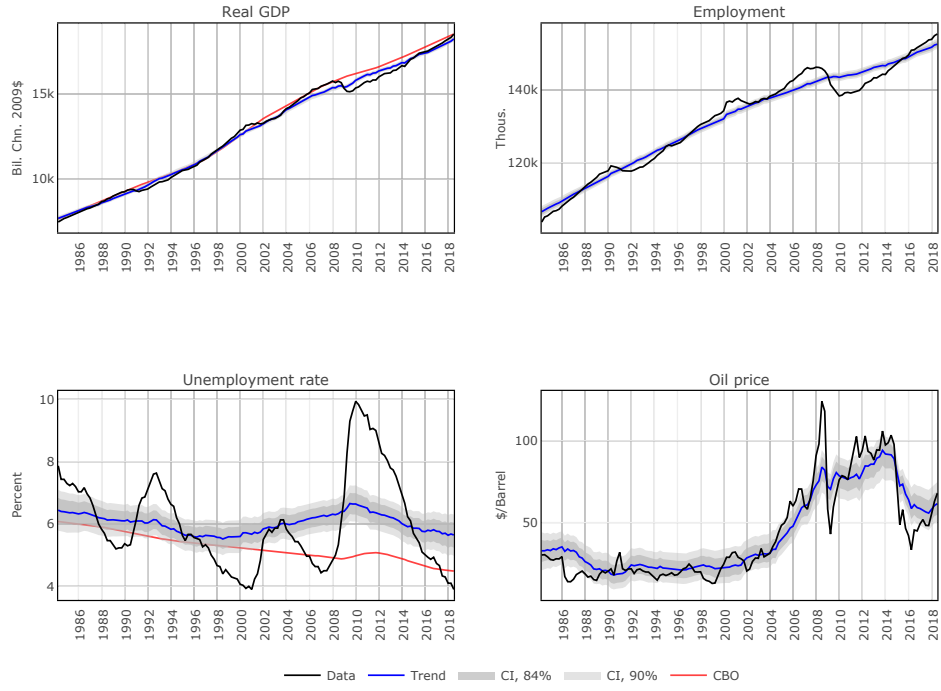

**Figure 20:** Independent trends of output, employment, unemployment, and oil prices (in blue), with coverage intervals at 68% coverage (dark shade) and 90% coverage (light shade), as estimated by the model. The chart also reports the measures of potential outputs and NAIRU estimated by the CBO (in red).

differences are equal to one. For this reason, we normalise  $\phi_\pi$ ,  $\phi_{\pi^c}$ ,  $\phi_{uom}$  and  $\phi_{spf}$  to the reciprocal of the standard deviation of the first difference of the respective variable.

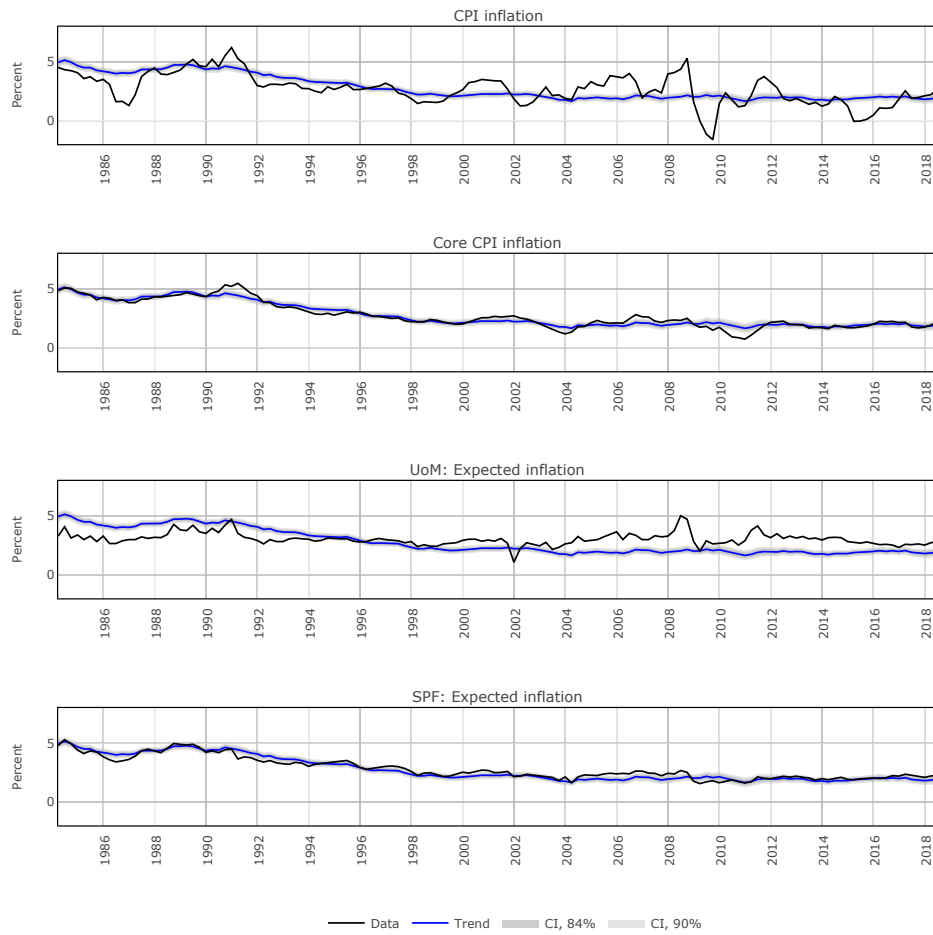

**Figure 21:** Trend common to CPI inflation, core CPI inflation, and inflation expectations (in blue), with coverage intervals at 68% coverage (dark shade) and 90% coverage (light shade), as estimated by the model.

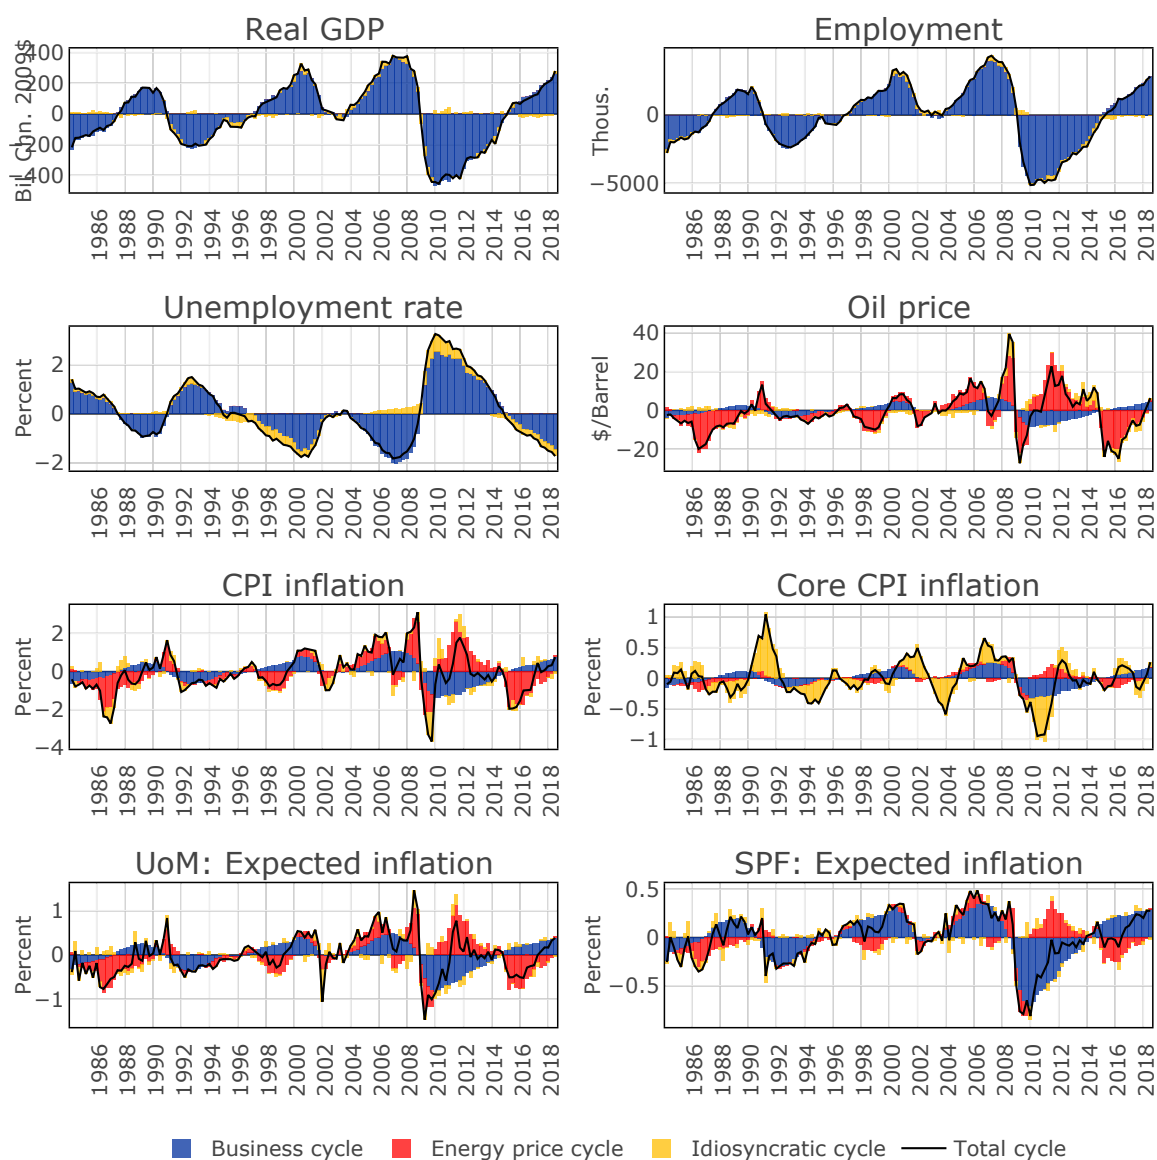

**Figure 22:** Historical decomposition of the cycles, as estimated by the model. The chart reports the Business cycle (in blue), Energy price cycle (in red), and idiosyncratic cycle (in yellow).



## Appendix E Employment-to-Population Ratio

The state-space model is identical to the one reported in the main text.

**Table 4:** Data and transformations

| Variable                       | Symbol                | Mnemonic | Transformation |
|--------------------------------|-----------------------|----------|----------------|
| Real GDP                       | $y_t$                 | $y$      | Levels         |
| Employment-to-population ratio | $e_t$                 | $e$      | Levels         |
| Unemployment rate              | $u_t$                 | $u$      | Levels         |
| Oil price                      | $oil_t$               | $oil$    | Levels         |
| CPI inflation                  | $\pi_t$               | $\pi$    | YoY            |
| Core CPI inflation             | $\pi_t^c$             | $\pi^c$  | YoY            |
| UoM: Expected inflation        | $F_t^{uom} \pi_{t+4}$ | $uom$    | Levels         |
| SPF: Expected CPI              | $F_t^{spf} \pi_{t+4}$ | $spf$    | Levels         |

**Note:** The table lists the macroeconomic variables used in the empirical model. ‘UoM: Expected inflation’ is the University of Michigan, 12-months ahead expected inflation rate. ‘SPF: Expected CPI’ is the Survey of Professional Forecasters, 4-quarters ahead expected CPI inflation rate. The oil price is the West Texas Intermediate Spot oil price.

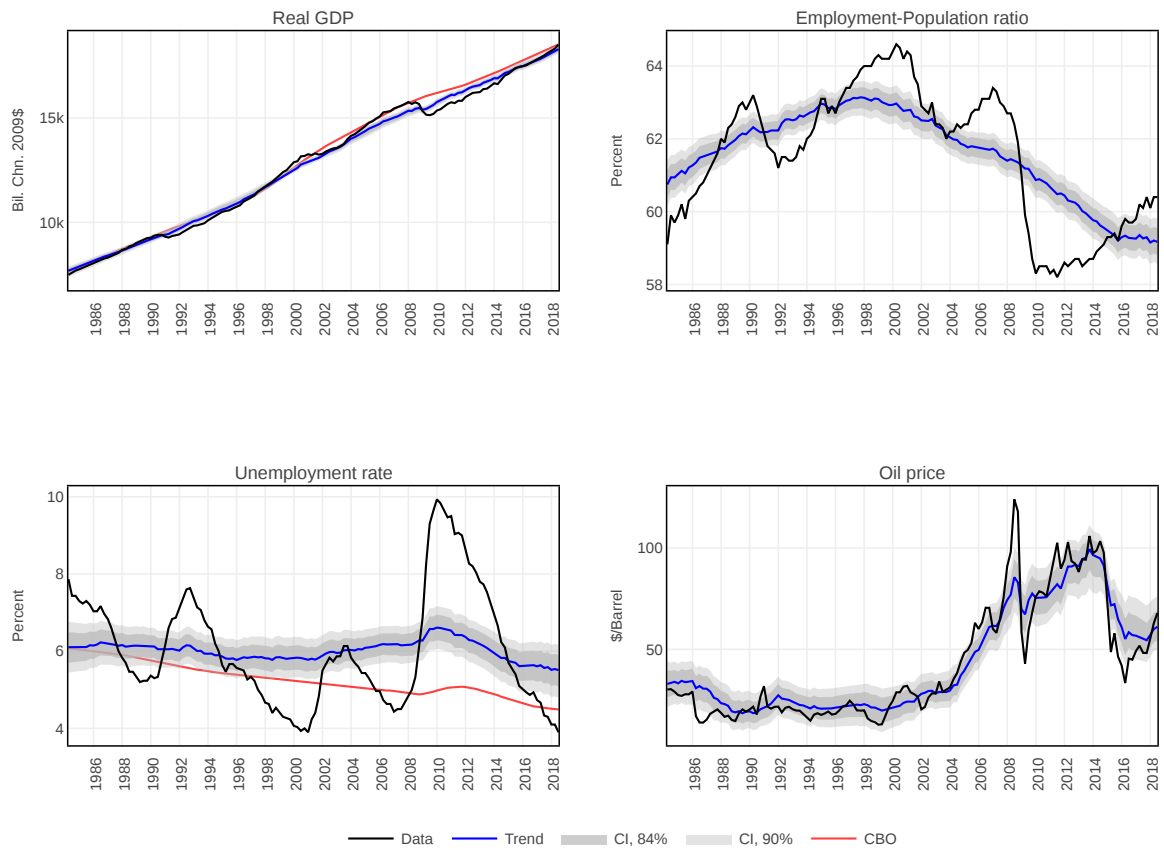

**Figure 23:** Independent trends of output, employment, unemployment, and oil prices (in blue), with coverage intervals at 68% coverage (dark shade) and 90% coverage (light shade), as estimated by the model. The chart also reports the measures of potential outputs and NAIRU estimated by the CBO (in red).

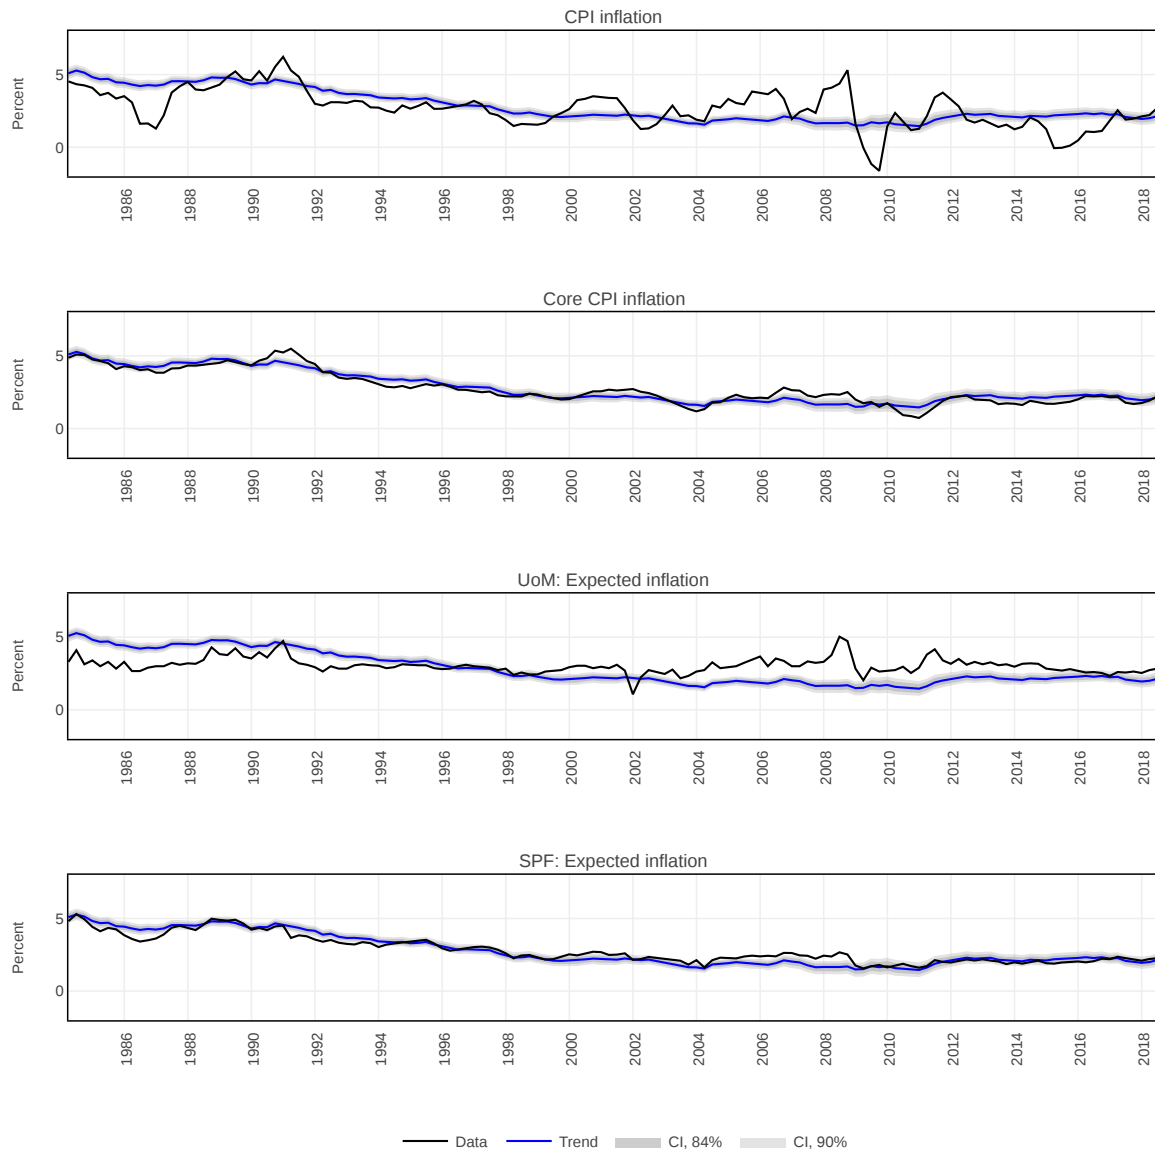

**Figure 24:** Trend common to CPI inflation, core CPI inflation, and inflation expectations (in blue), with coverage intervals at 68% coverage (dark shade) and 90% coverage (light shade), as estimated by the model.

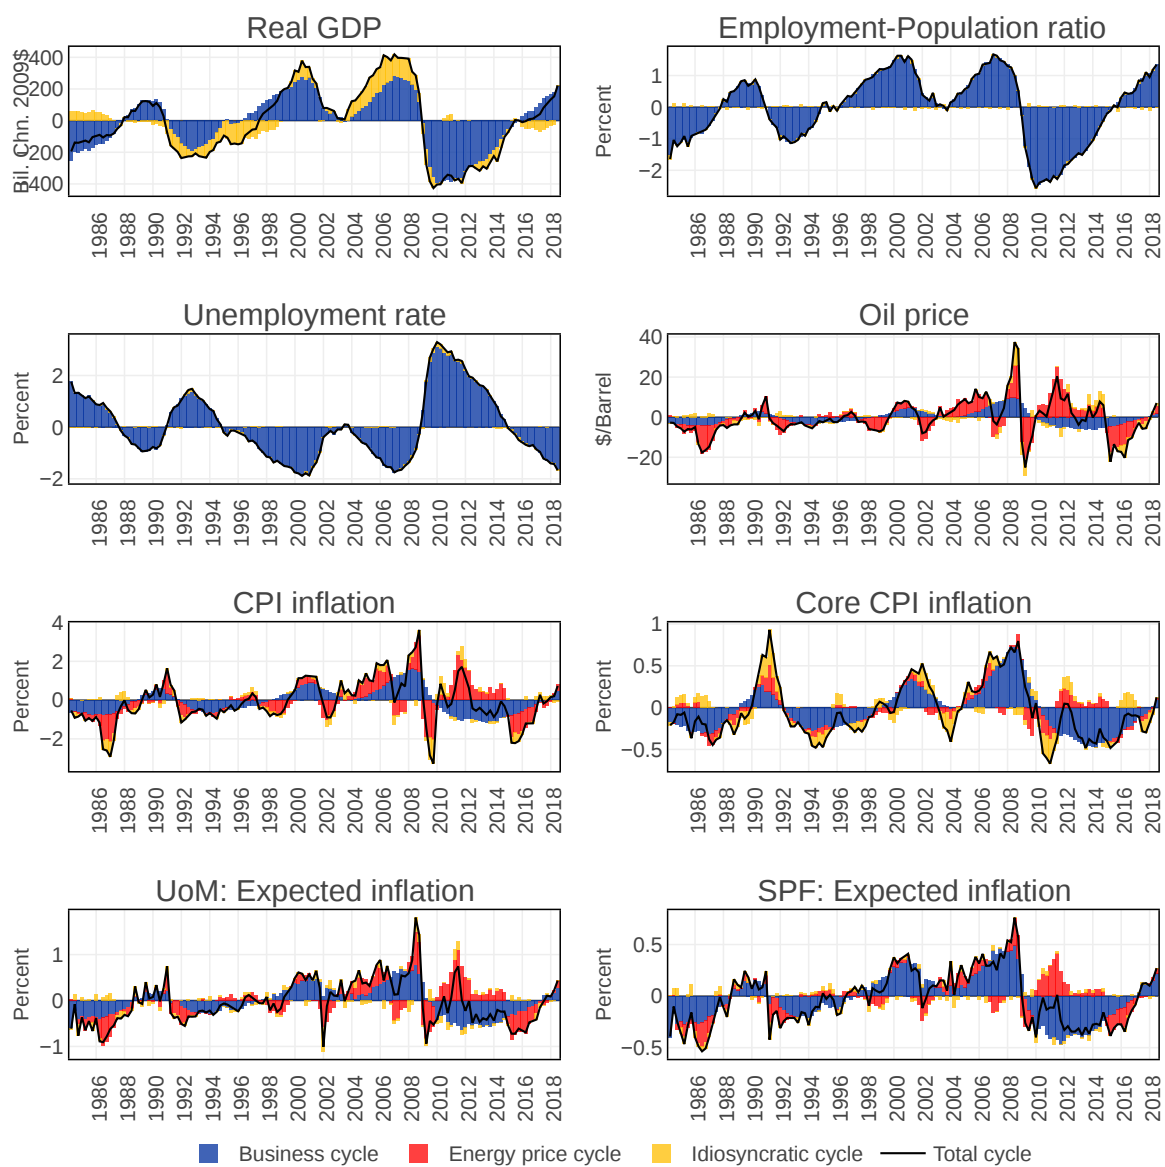

**Figure 25:** Historical decomposition of the cycles, as estimated by the model. The chart reports the Business cycle (in blue), Energy price cycle (in red), and idiosyncratic cycle (in yellow).

## Appendix F Global Activity

### F.1 Correlation of Cycles with Global Activity Indicators

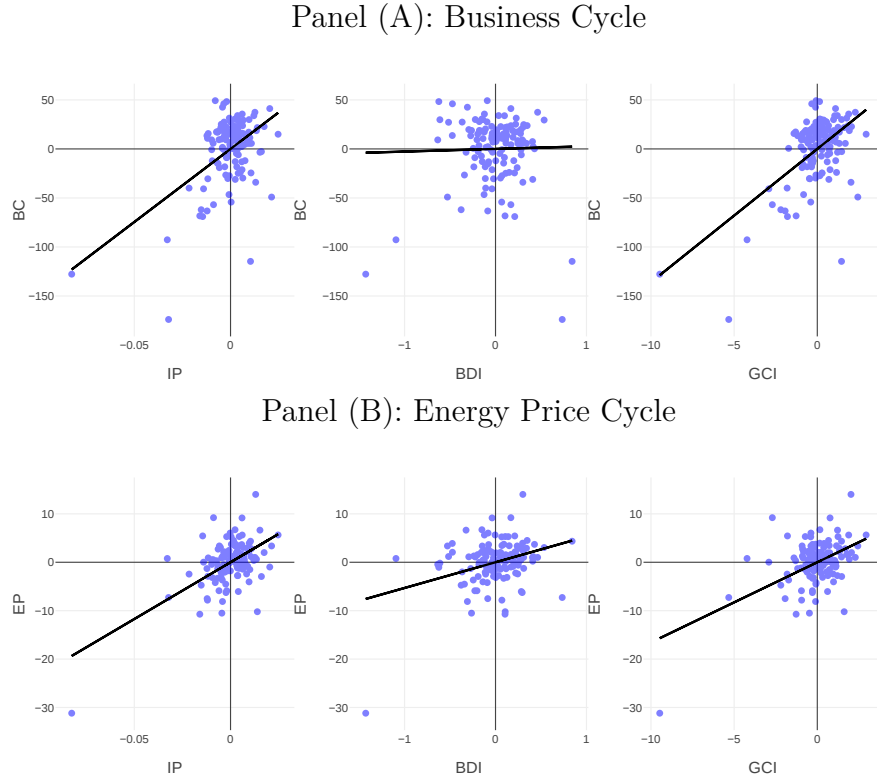

**Figure 26:** Scatter-plots and regression lines of the business cycle and the energy price cycle (differenced and standardised) on three global activity variables: (i) the Baltic Dry Index (BDI), initially proposed by [Kilian \(2009\)](#) but taken in level; (ii) the measure of global industrial production (GIP) proposed by [Baumeister and Hamilton \(2019\)](#) and based on the OECD methodology; and (iii) the Global Condition Index (GCI) of [Cuba-Borda et al. \(2018\)](#).

**Table 5:** Data and transformations

| Variable                     | Symbol                | Mnemonic | Transformation |
|------------------------------|-----------------------|----------|----------------|
| Real GDP                     | $y_t$                 | $y$      | Levels         |
| Employment                   | $e_t$                 | $e$      | Levels         |
| Unemployment rate            | $u_t$                 | $u$      | Levels         |
| Global industrial production | $ip_t$                | $ip$     | Levels         |
| Baltic Dry Index             | $bdi_t$               | $bdi$    | Levels         |
| Oil price                    | $oil_t$               | $oil$    | Levels         |
| CPI inflation                | $\pi_t$               | $\pi$    | YoY            |
| Core CPI inflation           | $\pi_t^c$             | $\pi^c$  | YoY            |
| UoM: Expected inflation      | $F_t^{uom} \pi_{t+4}$ | $uom$    | Levels         |
| SPF: Expected CPI            | $F_t^{spf} \pi_{t+4}$ | $spf$    | Levels         |

**Note:** The table lists the macroeconomic variables used in the empirical model. ‘UoM: Expected inflation’ is the University of Michigan, 12-months ahead expected inflation rate. ‘SPF: Expected CPI’ is the Survey of Professional Forecasters, 4-quarters ahead expected CPI inflation rate. The oil price is the West Texas Intermediate Spot oil price. The Baltic Dry Index is issued daily by the London-based Baltic Exchange as a proxy for global activity. Global industrial production was downloaded from James Hamilton’s webpage and it is part of the replication dataset of [Baumeister and Hamilton \(2019\)](#).

## F.2 A Model with Global Indicators

Our model in  $\tilde{x}_t := \{y_t, e_t, u_t, ip_t, bdi_t, oil_t, \pi_t, \pi_t^c, F_t^{uom} \pi_{t+4}, F_t^{spf} \pi_{t+4}\}$  can be written as

$$\begin{pmatrix} y_t \\ e_t \\ u_t \\ ip_t \\ bdi_t \\ oil_t \\ \pi_t \\ \pi_t^c \\ F_t^{uom} \pi_{t+4} \\ F_t^{spf} \pi_{t+4} \end{pmatrix} = \begin{pmatrix} 1 & 0 & 0 \\ \delta_{e,1} + \delta_{e,2}L & 0 & 0 \\ \delta_{u,1} + \delta_{u,2}L & 0 & 0 \\ \delta_{ip,1} + \delta_{ip,2}L & 1 & 0 \\ \delta_{bdi,1} + \delta_{bdi,2}L & \gamma_{bdi} & 0 \\ \delta_{oil,1} + \delta_{oil,2}L & \gamma_{oil,1} + \gamma_{oil,2}L & 0 \\ \delta_{\pi,1} + \delta_{\pi,2}L & \gamma_{\pi,1} + \gamma_{\pi,2}L & \phi_{\pi} \\ \delta_{\pi^c,1} + \delta_{\pi^c,2}L & \gamma_{\pi^c,1} + \gamma_{\pi^c,2}L & \phi_{\pi^c} \\ \delta_{uom,1} + \delta_{uom,2}L + \delta_{uom,3}L^2 & \gamma_{uom,1} + \gamma_{uom,2}L & \phi_{uom} \\ \delta_{spf,1} + \delta_{spf,2}L + \delta_{spf,3}L^2 & \gamma_{spf,1} + \gamma_{spf,2}L & \phi_{spf} \end{pmatrix} \begin{pmatrix} \hat{\psi}_t \\ \psi_t^{GD} \\ \mu_t^{\pi} \end{pmatrix} + \begin{pmatrix} \psi_t^y \\ \psi_t^e \\ \psi_t^u \\ \psi_t^{ip} \\ \psi_t^{bdi} \\ \psi_t^{oil} \\ \psi_t^{\pi} \\ \psi_t^{\pi^c} \\ \psi_t^{uom} \\ \psi_t^{spf} \end{pmatrix} + \begin{pmatrix} \mu_t^y \\ \mu_t^e \\ \mu_t^u \\ \mu_t^{ip} \\ \mu_t^{bdi} \\ \mu_t^{oil} \\ 0 \\ 0 \\ \mu_t^{uom} \\ \mu_t^{spf} \end{pmatrix} \quad (8)$$

where  $\phi_{\pi}$ ,  $\phi_{\pi^c}$ ,  $\phi_{uom}$ , and  $\phi_{spf}$  are normalised to have unitary loading of inflation and inflation expectations on trend inflation.<sup>6</sup>

<sup>6</sup>In the empirical model, the series are standardised so that the standard deviations of their first differences are equal to one. For this reason, we normalise  $\phi_{\pi}$ ,  $\phi_{\pi^c}$ ,  $\phi_{uom}$ , and  $\phi_{spf}$  to the reciprocal of the

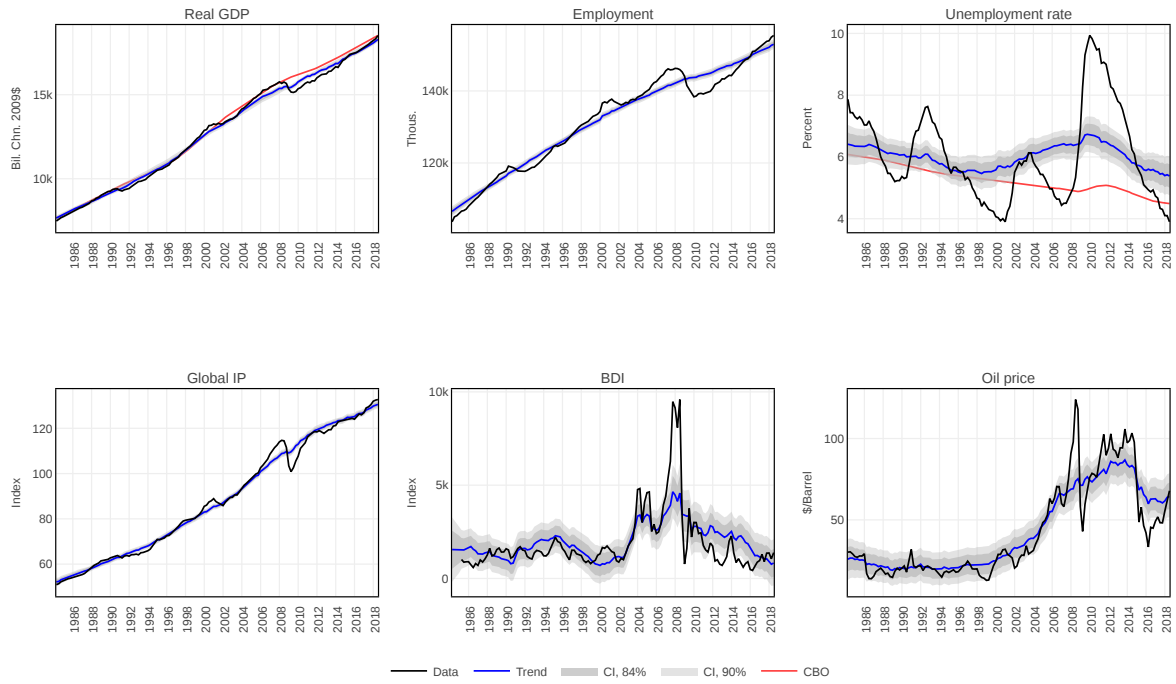

**Figure 27:** Independent trends of output, employment, unemployment, and oil prices (in blue), with coverage intervals at 68% coverage (dark shade) and 90% coverage (light shade), as estimated by the model. The chart also reports the measures of potential outputs and NAIRU estimated by the CBO (in red).

standard deviation of the first difference of the respective variable.

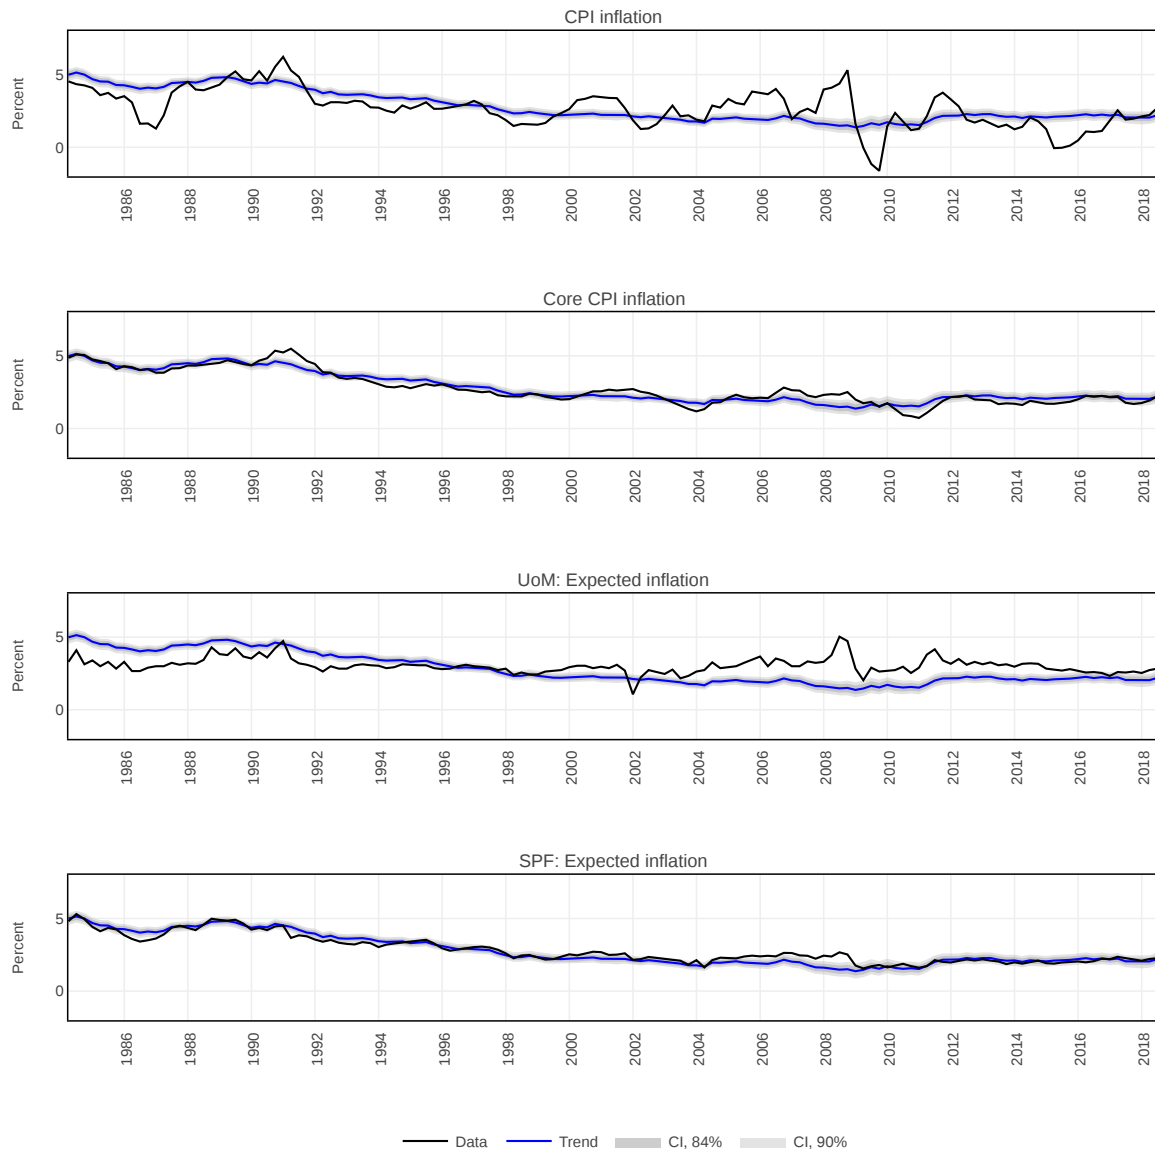

**Figure 28:** Trend common to CPI inflation, core CPI inflation, and inflation expectations (in blue), with coverage intervals at 68% coverage (dark shade) and 90% coverage (light shade), as estimated by the model.



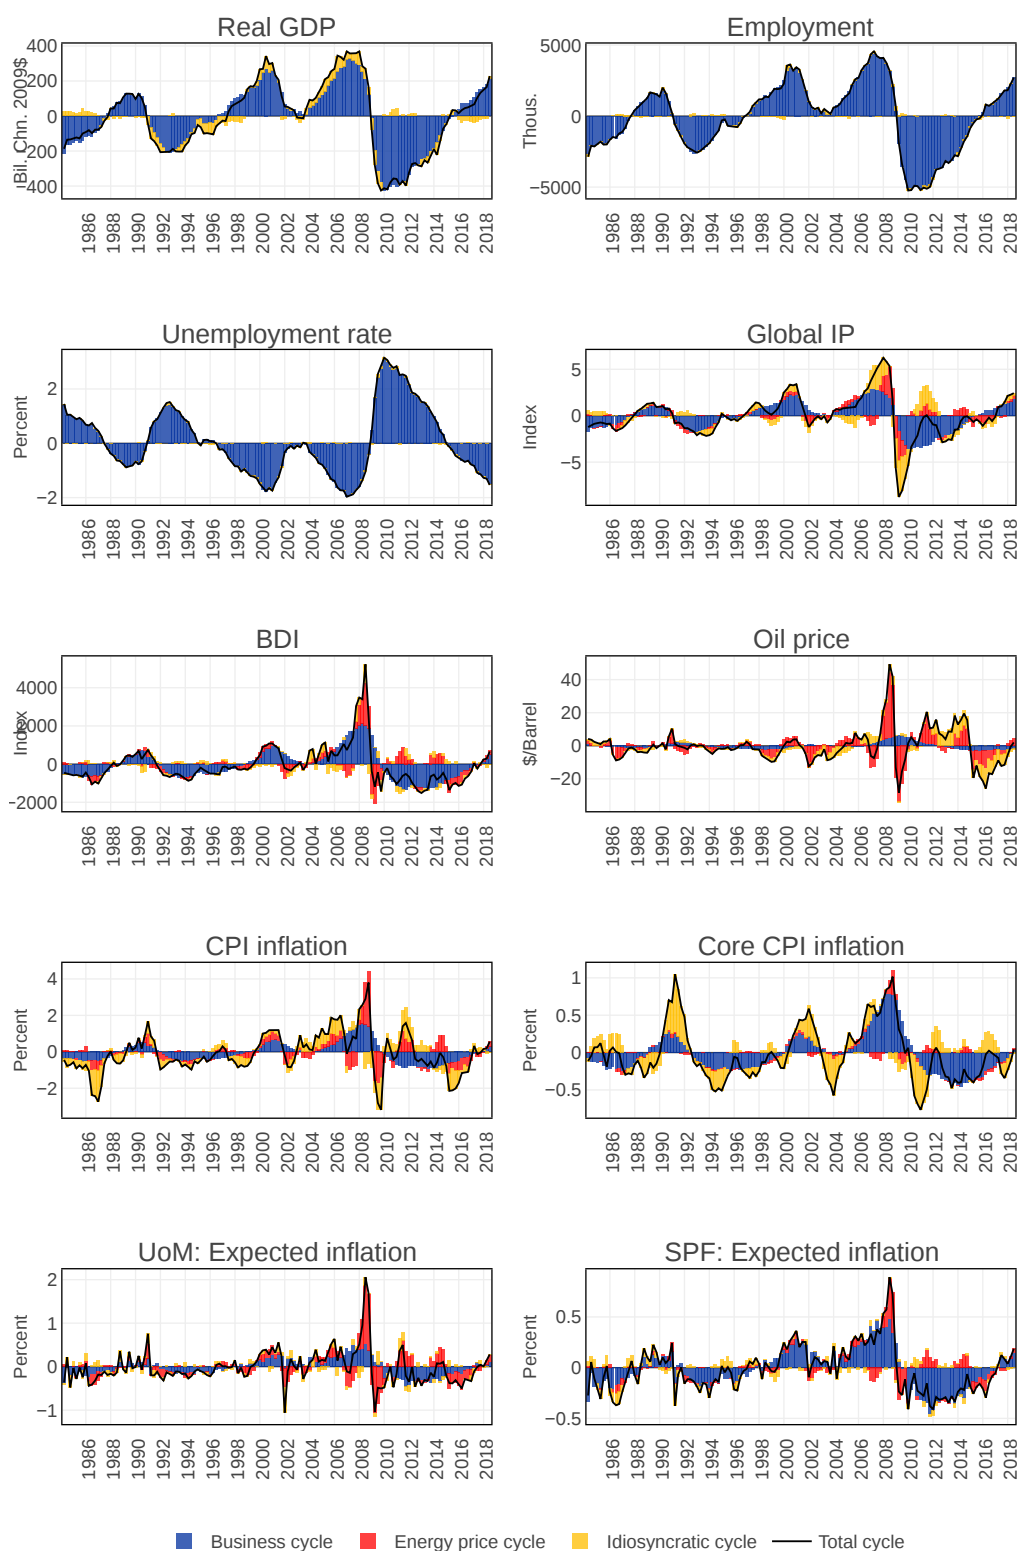

**Figure 29:** Historical decomposition of the cycles, as estimated by the model. The chart reports the Business cycle (in blue), Energy price cycle (in red), and idiosyncratic cycle (in yellow).

## Appendix G Priors for the Long-Run

In [section 7](#) we compare the forecast of the trend-cycle model with the forecast of a Bayesian VAR with the priors for the long run proposed in [Giannone et al. \(2019\)](#). Those priors require us to elicit a matrix  $H$  that captures the cointegration relationships between the variables in our information set  $\{y_t, e_t, u_t, oil_t, \pi_t, \pi_t^c, F_t^{uom} \pi_{t+4}, F_t^{spf} \pi_{t+4}\}$ . In the forecast exercise we adopt the following  $H$  matrix, in line with the assumptions made in the trend-cycle model:

$$H = \begin{pmatrix} 1 & 0 & 0 & 0 & 0 & 0 & 0 & 0 \\ 0 & 1 & 0 & 0 & 0 & 0 & 0 & 0 \\ 0 & 0 & 1 & 0 & 0 & 0 & 0 & 0 \\ 0 & 0 & 0 & 1 & 0 & 0 & 0 & 0 \\ 0 & 0 & 0 & 0 & 1 & 1 & 1 & 1 \\ 0 & 0 & 0 & 0 & -1 & 1 & 0 & 0 \\ 0 & 0 & 0 & 0 & -1 & 0 & 1 & 0 \\ 0 & 0 & 0 & 0 & -1 & 0 & 0 & 1 \end{pmatrix} \begin{array}{l} \leftarrow \text{Idio trend in GDP} \\ \leftarrow \text{Idio trend in Employment} \\ \leftarrow \text{Idio trend in Unemployment Rate} \\ \leftarrow \text{Idio trend in Oil prices} \\ \leftarrow \text{Common trend in inflation and expectations} \\ \leftarrow \text{CPI and core inflation are cointegrated} \\ \leftarrow \text{CPI and UoM expectations are cointegrated} \\ \leftarrow \text{CPI and SPF expectations are cointegrated} \end{array} \quad (9)$$

## References

- Baumeister, Christiane and James D Hamilton**, “Structural interpretation of vector autoregressions with incomplete identification: Revisiting the role of oil supply and demand shocks,” *American Economic Review*, 2019, *109* (5), 1873–1910.
- Beveridge, Stephen and Charles R Nelson**, “A new approach to decomposition of economic time series into permanent and transitory components with particular attention to measurement of the business cycle,” *Journal of Monetary Economics*, 1981, *7* (2), 151–174.
- Clark, Peter K**, “The cyclical component of US economic activity,” *The Quarterly Journal of Economics*, 1987, *102* (4), 797–814.
- Cuba-Borda, Pablo, Alexander Mechanick, and Andrea Raffo**, “Monitoring the World Economy : A Global Conditions Index,” IFDP Notes 2018-06-15, Board of Governors of the Federal Reserve System (U.S.) June 2018.
- Durbin, James and Siem Jan Koopman**, “A simple and efficient simulation smoother for state space time series analysis,” *Biometrika*, 2002, pp. 603–615.
- and — , *Time series analysis by state space methods*, Vol. 38, OUP Oxford, 2012.
- Giannone, Domenico, Michele Lenza, and Giorgio E. Primiceri**, “Priors for the Long Run,” *Journal of the American Statistical Association*, 2019, *114* (526), 565–580.
- Harvey, Andrew C**, “Trends and cycles in macroeconomic time series,” *Journal of Business & Economic Statistics*, 1985, *3* (3), 216–227.
- , **Thomas M Trimbur, and Herman K Van Dijk**, “Trends and cycles in economic time series: A Bayesian approach,” *Journal of Econometrics*, 2007, *140* (2), 618–649.
- Herbst, E.P. and F. Schorfheide**, *Bayesian Estimation of DSGE Models* The Econometric and Tinbergen Institutes Lectures, Princeton University Press, 2015.

- Jarociński, Marek**, “A note on implementing the Durbin and Koopman simulation smoother,” *Computational Statistics & Data Analysis*, 2015, *91*, 1–3.
- Kilian, Lutz**, “Not All Oil Price Shocks Are Alike: Disentangling Demand and Supply Shocks in the Crude Oil Market,” *American Economic Review*, June 2009, *99* (3), 1053–69.
- Koopman, Siem J and James Durbin**, “Fast filtering and smoothing for multivariate state space models,” *Journal of Time Series Analysis*, 2000, *21* (3), 281–296.
- Warne, Anders**, “YADA Manual,” *Manuscript*, December, 2008, 18.
